# Supplementary material for: A robust approach for estimating change-points in the mean of an AR(p) process
Source: arXiv:1509.00899 source file (2015-09-02)
Supplement: Supplementary file 1 [file supplement.tex]

\section{Proofs} \label{ar1:App:Proof}

\subsection{Proof of Proposition \ref{prop:corr_tcl}}\label{arp:proof:corr_tcl}
Since there is only a finite number of atypical values in the process $(x_i)$, 
Theorem 4 of \textcite{levy2011robust} still holds and gives that for all fixed $h\geq 1$:
\begin{equation*}%\label{eq:asym_exp_gamma}
\sqrt{n-h}\left(\frac{Q_{n}^2 \left(x^+_h\right) - Q_{n}^2 \left(x^-_h\right)}{4}-\gamma(h)\right)
=\frac{1}{\sqrt{n-h}}\sum_{i=1}^{n-h}\psi(\nu_i,\nu_{i+h})+o_P(1)\; ,
\end{equation*}
where $\gamma$ denotes the autocovariance of $(\nu_i)$ and where for all $x$ and $y$,

\begin{multline*}%\label{def:psi}
\psi : (x,y)\mapsto
\\ \left\{(\gamma(0)+\gamma(h)) \; \IF\left(\frac{x+y}{\sqrt{2(\gamma(0)+\gamma(h))}},Q,\Phi\right)
- (\gamma(0)-\gamma(h)) \; \IF\left(\frac{x-y}{\sqrt{2(\gamma(0)-\gamma(h))}},Q,\Phi\right)\right\}\; .
\end{multline*}

In this equation $\IF$ is defined by 

\begin{equation*}
\IF(x,Q,\Phi)
=c(\Phi)\left(\frac{1/4-\Phi(x+1/c(\Phi))
+\Phi(x-1/c(\Phi))}{\int_{\rset} \phi(y)\phi(y+1/c(\Phi))\rmd y}\right)\;,
\end{equation*}

where $c(\Phi)=1/(\sqrt{2}\Phi^{-1}(5/8))\approx 2.21914$, and $\Phi$ is here the cumulative distribution function of the standard normal distribution.
By Theorem 2 of \textcite{levy2011robust}, we obtain that 
$$
\frac{Q_{n}^2 \left(x^+_h\right) + Q_{n}^2 \left(x^-_h\right)}{4}-\gamma(0)=o_p(1)\;.
$$
Let $\widehat{\gamma}(0)=(Q_{n}^2 \left(x^+_h\right) + Q_{n}^2 \left(x^-_h\right))/4$ then

\begin{equation*}
\sqrt{n-h}\left(\widehat{\rho}(h)-\rho(h)\right)
=\frac{\widehat{\gamma}(0)^{-1}}{\sqrt{n-h}}\sum_{i=1}^{n-h}\psi(\nu_i,\nu_{i+h})+o_P(1)\; ,
\end{equation*}

In order to prove a central limit theorem for 
$\boldsymbol{\widehat{\rho}}_{1:(p+1)}$, it is enough to prove
by the Cramér-Wold device \parencite[Theorem 29.4]{billingsley1995probability}, that for any $a_k$ in $\rset$:
\begin{equation*}%\label{eq:CL_psi}
\frac{\widehat{\gamma}(0)^{-1}}{\sqrt{n}}\sum_{i=1}^{n-(p+1)}\sum_{k=1}^{p+1} a_k\psi(\nu_i,\nu_{i+k})
\end{equation*}
converges in distribution to a centered Gaussian rv. 
By Lemma 13 of \textcite{levy2011robust},
$\psi$ is of Hermite rank 2. Hence, the Hermite rank of the linear combination of the $\psi$ function is 
larger than 2. Thus, Condition (2.40) of Theorem 4 in \textcite{arcones1994limit} is satisfied
and the quantity $n^{-1/2}\sum_{i=1}^{n-(p+1)}\sum_{k=1}^{p+1} a_k\psi(\nu_i,\nu_{i+k})$ 
converges in distribution to a centered Gaussian rv with variance $\tilde{\sigma}^2$ given by
$$
\tilde{\sigma}^2=\PE\left[\left(\sum_{k=1}^{p+1} a_k\psi(\nu_1,\nu_{k+1})\right)^2\right]+2\sum_{\ell\geq 1}
\PE\left[\left(\sum_{k=1}^{p+1} a_k\psi(\nu_1,\nu_{k+1})\right)\left(\sum_{k=1}^{p+1} a_k\psi(\nu_{\ell+1},\nu_{k+\ell+1})\right)\right]\;.
$$
By Slutsky's lemma,
$
\sqrt{n-h}\left(\widehat{\rho}(h)-\rho(h)\right)
$
converges in distribution to a centered Gaussian rv with variance $\gamma(0)\tilde{\sigma}^2$.
Since $\left(x_i - \mathbb{E}x_i\right)$ is an ARMA($p$,1) process, with autoregressive parameters $\phi_1^\star, \dots ,\phi_p^\star$, 
we get, by \textcite[Chapter 11, Paragraph 2]{azencott}, that $R_p$, as defined in \eqref{eq:matrixR}, is invertible, and
\begin{equation*}
\Phi^\star = R_p^{-1}\boldsymbol{\rho}_{2:(p+1)}^T\;,
\end{equation*}
where $\boldsymbol{\rho}_{2:(p+1)}$ is defined in \eqref{eq:rho}.

Let $g:\mathcal{D}\subset\mathbb{R}^{p+1}\rightarrow\mathbb{R}^p$ defined by
\begin{equation}\label{eq:def_g}
g(u) = \left(u_{|j-i-1|}\mathbf{1}_{j-i-1\neq 0} + \mathbf{1}_{j-i-1=0}\right)_{1\leq i,j\leq p}^{-1}\left(u_2,\dots ,u_{p+1}\right)^T \; .
\end{equation}
Hence, 
\begin{eqnarray*}
\Phi^\star & = & g(\boldsymbol{\rho}_{1:(p+1)}) \; ,\\
\widetilde{\Phi}_n^{(p)} & = & g(\boldsymbol{\widetilde{\rho}_n}_{1:(p+1)})\; .
\end{eqnarray*}
By \eqref{eq:ANrho} and the delta method:
\begin{equation*}
\sqrt{n}\left(\widetilde{\Phi}_n^{(p)} - \Phi^\star\right) \underset{n\rightarrow\infty}{\rightarrow} \mathcal{N}\left(0, \nabla g (\boldsymbol{\rho}_{1:(p+1)})^T V \nabla g (\boldsymbol{\rho}_{1:(p+1)})\right) \; ,
\end{equation*}
$\nabla g (\boldsymbol{\rho}_{1:(p+1)})$ being the Jacobian matrix of $g$ in $\boldsymbol{\rho}_{1:(p+1)}$. Let us determine $\nabla g (u)\cdot h$ for all $u\in\mathcal{D},h\in\mathbb{R}^{p+1}$. Using \eqref{eq:def_g}, we get
\begin{equation*}
\left(h_{|j-i-1|}\mathbf{1}_{j-i-1\neq 0}\right)_{1\leq i,j\leq p}g(u) + \left(u_{|j-i-1|}\mathbf{1}_{j-i-1\neq 0} + \mathbf{1}_{j-i-1=0}\right)_{1\leq i,j\leq p}\nabla g(u)\cdot h = \left( h_2,\dots ,h_{p+1}\right)^T \; .
\end{equation*}
Applied to $u=\boldsymbol{\rho}_{1:(p+1)}$, we have
\begin{equation*}
R_p \nabla g \left(\boldsymbol{\rho}_{1:(p+1)} \right)\cdot h = \left(h_{j+1} - \sum_{j=1}^i \phi_{i+1-j}^\star h_j + \sum_{j=1}^{p-i-1}\phi_{i+j+1}^\star h_j\right)_{1\leq j \leq p} \; ,
\end{equation*}
and then $\nabla g \left(\boldsymbol{\rho}_{1:(p+1)}\right) = R_p^{-1}M$, where $M$ is defined in \eqref{eq:Jacobian}.

%%% Local Variables:
%%% mode: latex
%%% TeX-master: "arp.tex"
%%% End:

\subsection{Proof of Proposition \ref{Prop:Segment}}\label{subsec:prop:Segment}

In the sequel, we need the following definitions, notations and remarks. Observe that \eqref{eq:bkw} can be rewritten as follows:
\begin{equation}\label{eq:modele_matriciel}
z = \sum_{r=1}^p \phi_r^\star B^r z + T\left(\boldsymbol{t}_n^\star\right) \boldsymbol{\delta}^\star + \epsilon\;,
\end{equation}
where
\begin{equation}\label{eq:YXE}
z = \left( \begin{array}{c} z_1 \\\vdots \\z_{n} \end{array}\right)\;,
\qquad
B^r z = \left( \begin{array}{c} z_{1-r} \\ \vdots \\ z_{n-r} \end{array}\right)\;, 
\qquad
\boldsymbol{\delta}^\star = \left( \begin{array}{c} \delta^\star_0 \\ \vdots \\ \delta^\star_{m} \end{array}\right)\;, 
\qquad 
\epsilon = \left( \begin{array}{c} \epsilon_1 \\ \vdots \\ \epsilon_n \end{array}\right)\;,
\end{equation}
where $\delta_k^\star = (1-\sum_{r=1}^p\phi_r^\star) \mu^\star_k$, for $0 \leq k \leq m$,
and $T\left(\boldsymbol{t}\right)$ is an $n \times (m+1)$ matrix where the $k$th column is $( \underset{t_{k-1}}{\underbrace{0,\dots , 0}} \; \underset{t_k-t_{k-1}}{\underbrace{1,\dots ,1}} \; \underset{n - t_k}{\underbrace{0,\dots ,0}} )^T$.

Let us define the exact and estimated decorrelated series by
\begin{eqnarray}\label{eq:decor}
w^\star & = & z - \sum_{r=1}^p\phi_r^\star B^r z\;, \\
\overline{w} & = & z - \sum_{r=1}^p\overline{\phi}_{r,n} B^r z\label{eq:overline_x}\;.
\end{eqnarray}
where $\overline{\Phi}_n = \left(\phi_{r,n}\right)_{1\leq r\leq p}$.

For any vector subspace $E$ of $\mathbb{R}^{n}$, let $\pi_E$ denote the orthogonal projection of $\mathbb{R}^{n}$ on $E$.
Let also $\Vert \cdot \Vert$ be the Euclidean norm on $\mathbb{R}^{n}$, $\langle \cdot , \cdot \rangle$ the canonical scalar product on  $\mathbb{R}^{n}$ and 
$\Vert \cdot \Vert_{\infty}$ the sup norm. 

For $x$ a vector of $\rset^n$ and $\boldsymbol{t}\in\mathcal{A}_{n,m}$, let

\begin{equation}\label{eq:Jnm}
J_{n,m}\left(x,\boldsymbol{t}\right)
= \frac{1}{n} \left( \Vert \pi_{E_{ \boldsymbol{t}_n^\star } }\left( x\right) \Vert^2 - \Vert \pi_{ E_{\boldsymbol{t}}} \left( x \right) \Vert^2 \right)\;,
\end{equation}
written $J_n\left(x,\boldsymbol{t}\right)$ in the sequel for notational simplicity. In \eqref{eq:Jnm}, $E_{\boldsymbol{t}_n^\star}$ and $E_{\boldsymbol{t}}$ correspond to the
linear subspaces of $\mathbb{R}^{n}$ generated by the columns of $T\left(\boldsymbol{t}_n^\star\right)$ and $T\left(\boldsymbol{t}\right)$, respectively. We shall use the same decomposition
as the one introduced in \textcite{LM}:
\begin{equation}\label{eq:Jn_decomp}
J_n\left(x,\boldsymbol{t}\right) =  K_n\left(x,\boldsymbol{t}\right) + V_n\left(x,\boldsymbol{t}\right) + W_n\left(x,\boldsymbol{t}\right)\;,
\end{equation}
where
\begin{eqnarray*}
K_n\left(x,\boldsymbol{t}\right) & = & \frac{1}{n}\left\Vert \left(\pi_{E_{\boldsymbol{t}_n^\star}}- \pi_{E_{\boldsymbol{t}}}\right)\mathbb{E}x\right\Vert^2\;, \\
V_n\left(x,\boldsymbol{t}\right) & = & \frac{1}{n}\left(\left\Vert \pi_{E_{\boldsymbol{t}_n^\star}} \left( x-\mathbb{E}x\right)\right\Vert^2 - \left\Vert \pi_{E_{\boldsymbol{t}}} \left( x-\mathbb{E}x\right)\right\Vert^2\right)\;, \\
W_n\left(x,\boldsymbol{t}\right) & = & \frac{2}{n}\left( \left\langle \pi_{E_{\boldsymbol{t}_n^\star}} \left( x-\mathbb{E}x\right), \pi_{E_{\boldsymbol{t}_n^\star}} \left( \mathbb{E}x \right)\right\rangle - \left\langle \pi_{E_{\boldsymbol{t}}} \left( x-\mathbb{E}x\right), \pi_{E_{\boldsymbol{t}}} \left( \mathbb{E}x \right)\right\rangle  \right)\;.
\end{eqnarray*}

We shall also use the following notations:
\begin{eqnarray}
\underline{\lambda} & = & \underset{1\leq k\leq m}{\min} \left\vert \delta_k^\star-\delta_{k-1}^\star \right\vert\;,\label{eq:underline_lambda}\\
\overline{\lambda} & = & \underset{1\leq k\leq m}{\max} \left\vert \delta_k^\star-\delta_{k-1}^\star \right\vert\;,\label{eq:overline_lambda}\\
\Delta_{\boldsymbol{\tau}^\star} & = & \underset{1\leq k\leq m+1}{\min} \left(\tau_k^\star - \tau_{k-1}^\star\right)\;,\label{eq:Delta_tau*}\\
\mathcal{C}_{\alpha,\gamma,n} & = & \left\lbrace \boldsymbol{t} \in \mathcal{A}_{n,m}; \alpha\underline{\lambda}^{-2}\leq \Vert \boldsymbol{t} - \boldsymbol{t}_n^\star\Vert\leq n\gamma\Delta_{\boldsymbol{\tau}^\star}\right\rbrace\;,\label{eq:C_alpha_gamma_n}\\
\mathcal{C}_{\alpha,\gamma,n}' & = & \mathcal{C}_{\alpha,\gamma,n}\cap \left\lbrace \boldsymbol{t}\in\mathcal{A}_{n,m}; \forall k = 1,\dots, m, t_k\geq t_{n,k}^\star\right\rbrace\;,
\label{eq:C'_alpha_gamma_n} \\
\mathcal{C}_{\alpha,\gamma,n}'\left(\mathcal{I}\right) & = & \left\lbrace \boldsymbol{t}\in \mathcal{C}_{\alpha,\gamma,n}' ; \right. \nonumber\\
 & & \left. \forall k\in\mathcal{I}, \alpha\underline{\lambda}^{-2}\leq t_k - t_{n,k}^\star\leq n\gamma\Delta_{\boldsymbol{\tau}^\star} \textit{ and } \forall k\notin \mathcal{I}, t_k - t_{n,k}^\star < \alpha\underline{\lambda}^{-2}\right\rbrace\label{eq:C'alpha_gamma_n_I}\;,
\end{eqnarray}
for any $\alpha>0$, $0<\gamma <1/2$ and $\mathcal{I}\subset\left\lbrace 1,\dots ,m\right\rbrace$.
We shall also need the following lemmas in order to prove Proposition \ref{Prop:Segment} which are proved below.
\begin{lemma}\label{lem:rateXY}
Let $\left(z_{1-p} ,\dots ,z_n\right)$ be defined by \eqref{eq:modele_new} or \eqref{eq:bkw}, then, for all $r=0,\dots ,p$:
\begin{equation*}%\label{eq:rateXY}
\Vert B^r z \Vert = O_P\left(n^{1/2}\right)\;,
\end{equation*}
as $n$ tends to infinity, where $B^r z$ is defined in \eqref{eq:YXE}.
\end{lemma}

\begin{lemma}\label{lem:BoundedUnifBound}
Let $\left(z_{1-p} ,\dots ,z_n\right)$ be defined by \eqref{eq:modele_new} or \eqref{eq:bkw} then,
for all $\boldsymbol{t}\in\mathcal{A}_{n,m}$,
\begin{equation*}
\left\vert J_n \left(\overline{w}, \boldsymbol{t}\right) - J_n \left(w^\star, \boldsymbol{t}\right)\right\vert \leq \frac{2}{n} \sum_{r=1}^p \left| \phi_r^\star-\overline{\phi}_{r,n}\right|\left\Vert B^r z \right\Vert \left(p\left| \phi_r^\star-\overline{\phi}_{r,n}\right|\left\Vert B^r z \right\Vert + 2 \left\Vert w^\star\right\Vert\right) = O_P \left(n^{-1/2}\right) \;,
\end{equation*}
where $J_n$ is defined in \eqref{eq:Jnm}, $Bz$ and $z$ are defined in \eqref{eq:YXE}, $w^\star$ is defined in \eqref{eq:decor} and $\overline{w}$ is defined in \eqref{eq:overline_x}.
\end{lemma}

\begin{lemma}\label{lem:consistency}
Under the assumptions of Proposition \ref{Prop:Segment},
$\Vert\boldsymbol{\overline{\tau}_n}-\boldsymbol{\tau}^\star\Vert_{\infty}$ converges in probability to $0$, as $n$ tends to infinity.
\end{lemma}

\begin{lemma}\label{lem:almost72LM}
Under the assumptions of Proposition \ref{Prop:Segment} and for any $\alpha>0$, $0<\gamma <1/2$ and $\mathcal{I}\subset\left\lbrace 1,\dots ,m\right\rbrace$, 
\begin{equation*}
P\left(\min_{\boldsymbol{t}\in \mathcal{C}_{\alpha,\gamma,n}'\left(\mathcal{I}\right)} \left(\frac{1}{2} K_n\left(w^\star,\boldsymbol{t}\right) + V_n\left(w^\star,\boldsymbol{t}\right) + W_n\left(w^\star,\boldsymbol{t}\right)\right)\leq 0 \right) \longrightarrow 0\;,\; \textrm{as } n\to\infty\;,
\end{equation*}
where $\mathcal{C}_{\alpha,\gamma,n}'\left(\mathcal{I}\right)$ is defined in \eqref{eq:C'alpha_gamma_n_I} and $w^\star$ is defined in \eqref{eq:decor}.
\end{lemma}

\begin{lemma}\label{lem:almost72LM2}
Under the assumptions of Proposition \ref{Prop:Segment} and for any $\alpha>0$, $0<\gamma <1/2$ and $\mathcal{I}\subset\left\lbrace 1,\dots ,m\right\rbrace$, 
\begin{equation*}
P\left(\min_{\boldsymbol{t}\in \mathcal{C}_{\alpha,\gamma,n}'\left(\mathcal{I}\right)} J_n\left(\overline{w},\boldsymbol{t}\right)\leq 0\right) \longrightarrow 0
\;,\; \textrm{as } n\to\infty\;,
\end{equation*}
where $\mathcal{C}_{\alpha,\gamma,n}'\left(\mathcal{I}\right)$ is defined in \eqref{eq:C'alpha_gamma_n_I} and $\overline{w}$ is defined in \eqref{eq:overline_x}.
\end{lemma}

\begin{lemma}\label{lem:rateT}
Under the assumptions of Proposition \ref{Prop:Segment},
\begin{equation*}
\Vert\boldsymbol{\widehat{\tau}_n}(z, \overline{\Phi}_n)-\boldsymbol{\tau}^\star \Vert_{\infty} = O_P\left(n^{-1}\right)\;.
\end{equation*}
\end{lemma}

\begin{proof}[Proof of Lemma \ref{lem:rateXY}]
Without loss of generality, assume $\left(z_{1-p} ,\dots ,z_n \right)$ is defined by \eqref{eq:bkw}. %
$
\Vert B^r z\Vert^2 = \sum_{i=1-r}^{n-r}z_i^2 %\leq 2 \sum_{i=1-r}^{n-r}(z_i-\PE(z_i))^2+2 \sum_{i=1-r}^{n-r}\PE(z_i)^2.
$
then Markov inequality implies that
$
\Vert B^r z\Vert^2=O_P (n).
$
\end{proof}

\begin{proof}[Proof of Lemma \ref{lem:BoundedUnifBound}]
By \eqref{eq:decor}, $\overline{w}=w^\star+\sum_{r=1}^p(\phi_r^\star-\overline{\phi}_{r,n})B^r z$. 
We get
\begin{multline*}%\label{eq:Jnm_diff}
\left\Vert \pi_{E_{\boldsymbol{t}}} (\overline{w})\right\Vert^2 - \left\Vert \pi_{E_{\boldsymbol{t}}} (w^\star)\right\Vert^2 = 
\left\Vert \pi_{E_{\boldsymbol{t}}} (w^\star) + \sum_{r=1}^p(\phi_r^\star-\overline{\phi}_{r,n})\pi_{E_{\boldsymbol{t}}} (B^r z)\right\Vert^2 - \left\Vert \pi_{E_{\boldsymbol{t}}} (w^\star)\right\Vert^2 \\
=  \left\Vert \sum_{r=1}^p(\phi_r^\star-\overline{\phi}_{r,n})\pi_{E_{\boldsymbol{t}}} (B^r z)\right\Vert^2 + 2 \sum_{r=1}^p (\phi_r^\star-\overline{\phi}_{r,n})\left\langle \pi_{E_{\boldsymbol{t}}} (w^\star), \pi_{E_{\boldsymbol{t}}} (B^r z)\right\rangle \\
 \leq \sum_{r=1}^p p(\phi_r^\star-\overline{\phi}_{r,n})^2\left\Vert \pi_{E_{\boldsymbol{t}}} (B^r z)\right\Vert^2 + 2 \sum_{r=1}^p (\phi_r^\star-\overline{\phi}_{r,n})\left\langle \pi_{E_{\boldsymbol{t}}} (w^\star), \pi_{E_{\boldsymbol{t}}} (B^r z)\right\rangle \\
 \leq \sum_{r=1}^p  (\phi_r^\star-\overline{\phi}_{r,n}) \left(p(\phi_r^\star-\overline{\phi}_{r,n}) \left\Vert \pi_{E_{\boldsymbol{t}}} (B^r z)\right\Vert^2 + 2 \left\langle \pi_{E_{\boldsymbol{t}}} (w^\star), \pi_{E_{\boldsymbol{t}}} (B^r z)\right\rangle\right) \\
 \leq \sum_{r=1}^p  (\phi_r^\star-\overline{\phi}_{r,n}) \left\langle \pi_{E_{\boldsymbol{t}}} (B^r z) , p(\phi_r^\star-\overline{\phi}_{r,n}) \pi_{E_{\boldsymbol{t}}} (B^r z) + 2\pi_{E_{\boldsymbol{t}}} (w^\star)\right\rangle  \;.
\end{multline*}

The Cauchy-Schwarz inequality and the $1$-Lipschitz property of projections give
\begin{equation*}
\left|\left\Vert \pi_{E_{\boldsymbol{t}}} (\overline{w})\right\Vert^2 - \left\Vert \pi_{E_{\boldsymbol{t}}} (w^\star)\right\Vert^2 \right| \leq \sum_{r=1}^p \left| \phi_r^\star-\overline{\phi}_{r,n}\right|\left\Vert B^r z \right\Vert \left(p\left| \phi_r^\star-\overline{\phi}_{r,n}\right|\left\Vert B^r z \right\Vert + 2 \left\Vert w^\star\right\Vert\right)
\end{equation*}
The conclusion follows from \eqref{eq:Jnm}, \eqref{eq:hypRhoRate} and Lemma \ref{lem:rateXY}.
\end{proof}

\begin{proof}[Proof of Lemma \ref{lem:consistency}]
\textcite[proof of Theorem 3]{LM} give the following bounds for any $\boldsymbol{t} \in\mathcal{A}_{n,m} $:
\begin{eqnarray}\label{eq:LMbounds}
K_n\left(w^\star,\boldsymbol{t} \right) & \geq & \underline{\lambda}^2 \min\left(\frac{1}{n}\max_{1\leq k \leq m}\left\vert t_k - t_{n,k}^\star\right\vert , \Delta_{\boldsymbol{\tau}^\star}\right)\;,\\
V_n\left(w^\star,\boldsymbol{t}\right) & \geq & -\frac{2\left(m+1\right)}{n\Delta_n}\left(\max_{1\leq s\leq n} \left(\sum_{i=1}^s \epsilon_i\right)^2 + \max_{1\leq s\leq n} \left(\sum_{i=n-s}^{n} \epsilon_i\right)^2\right)\;,\\
\left\vert  W_n\left(w^\star,\boldsymbol{t} \right) \right\vert & \leq & \frac{3\left(m+1\right)^2 \overline{\lambda}}{n} \left(\max_{1\leq s\leq n} \left\vert\sum_{i=1}^s \epsilon_i\right\vert + \max_{1\leq s\leq n} \left\vert \sum_{i=n-s}^{n} \epsilon_i\right\vert \right)\;,
\end{eqnarray}
where $\underline{\lambda}$, $\overline{\lambda}$ anf $\Delta_{\boldsymbol{\tau}^\star}$ are defined in~(\ref{eq:underline_lambda}--\ref{eq:Delta_tau*}).
For any $\alpha>0$, define, as in the proof of Theorem~3 of \textcite{LM},
\begin{equation}\label{eq:Cn_alpha}
\mathcal{C}_{n,\alpha} = \left\lbrace \boldsymbol{t}\in \mathcal{A}_{n,m} ; \left\Vert \boldsymbol{t} - \boldsymbol{t}_{n}^\star\right\Vert_{\infty} \geq n\alpha\right\rbrace \;.
\end{equation}
For $0<\alpha<\Delta_{\boldsymbol{\tau}^\star}$, we have:
\begin{eqnarray*}
P\left(\left\Vert \boldsymbol{\widehat{t}}_n(z, \overline{\Phi}_n) - \boldsymbol{t}_{n}^\star \right\Vert_{\infty} \geq n\alpha\right)  & \leq & P \left( \min_{\boldsymbol{t}\in\mathcal{C}_{n,\alpha}} J_n \left(\overline{w}, \boldsymbol{t} \right) \leq 0\right)\\
 & \leq &P \left( \min_{\boldsymbol{t}\in\mathcal{C}_{n,\alpha}} \left(J_n \left(\overline{w}, \boldsymbol{t} \right) - J_n \left(w^\star, \boldsymbol{t}\right) \right)\leq -\alpha\underline{\lambda}^2 \right)\\
 & + & P \left( \min_{\boldsymbol{t}\in\mathcal{C}_{n,\alpha}} \left(V_n\left(w^\star, \boldsymbol{t}\right) + W_n\left(w^\star, \boldsymbol{t}\right)\right) \leq  -\alpha\underline{\lambda}^2 \right) \\
 & \leq & P \left( \min_{\boldsymbol{t}\in\mathcal{C}_{n,\alpha}} \left(J_n \left(\overline{w}, \boldsymbol{t} \right) - J_n \left(w^\star, \boldsymbol{t} \right)\right)\leq -\alpha\underline{\lambda}^2 \right)\\
 & + & P \left( \max_{1\leq s\leq n}{\left(\sum_{i=1}^s \epsilon_i\right)^2} + \max_{1 \leq s \leq n} \left(\sum_{i=n-s}^{n} \epsilon_i\right)^2 \geq c\underline{\lambda}^2 n\Delta_n \alpha \right)\\
 & + & P \left( \max_{1 \leq s \leq n}{\left\vert\sum_{i=1}^s \epsilon_i\right\vert} + \max_{1 \leq s \leq n} \left\vert\sum_{i=n-s}^{n} \epsilon_i\right\vert \geq c\underline{\lambda}^2 n \alpha \overline{\lambda}^{-1} \right)
\end{eqnarray*}
for some positive constant $c$. The last two terms of this sum go to $0$ when $n$ goes to infinity~\parencite[proof of Theorem 3]{LM}. To show that the first term shares the same property, it suffices to show that $J_n \left(\overline{w}, \boldsymbol{t}\right) - J_n\left(w^\star,\boldsymbol{t}\right)$ is bounded uniformly in $\boldsymbol{t}$ by a sequence of rv's which converges to $0$ in probability. This result holds by Lemma \ref{lem:BoundedUnifBound}.
\end{proof}

\begin{proof}[Proof of Lemma \ref{lem:almost72LM}]
Using \textcite[Equations (64--66)]{LM}, one can show the bound (73) of \textcite{LM} on 
$$P\left(\min_{\boldsymbol{t}\in \mathcal{C}_{\alpha,\gamma,n}'\left(\mathcal{I}\right)} \left(K_n\left(w^\star,\boldsymbol{t}\right) + V_n\left(w^\star,\boldsymbol{t}\right) + W_n\left(w^\star,\boldsymbol{t}\right)\right)\leq 0 \right).$$
 Using the same arguments, we have the same bound on 
$$P\left(\min_{\boldsymbol{t} \in \mathcal{C}_{\alpha,\gamma,n}'\left(\mathcal{I}\right)} \left(\frac{1}{2} K_n\left(w^\star,\boldsymbol{t} \right) + V_n\left(w^\star,\boldsymbol{t} \right) + W_n\left(w^\star,\boldsymbol{t} \right)\right)\leq 0 \right).$$
We conclude using \textcite[Equations (67--71)]{LM}.
\end{proof}

\begin{proof}[Proof of Lemma \ref{lem:almost72LM2}]
By (\ref{eq:Jn_decomp}),
\begin{multline*}
P\left(\min_{\boldsymbol{t}\in \mathcal{C}_{\alpha,\gamma,n}'\left(\mathcal{I}\right)} J_n\left(\overline{w},\boldsymbol{t}\right)\leq 0\right)
\leq P\left(\min_{\boldsymbol{t}\in \mathcal{C}_{\alpha,\gamma,n}'\left(\mathcal{I}\right)} \left(J_n\left(\overline{w},\boldsymbol{t}\right) - J_n\left(w^\star,\boldsymbol{t}\right) + \frac{1}{2} K_n\left(w^\star,\boldsymbol{t}\right)\right)\leq 0\right)\\
 +  P\left(\min_{\boldsymbol{t}\in \mathcal{C}_{\alpha,\gamma,n}'\left(\mathcal{I}\right)} \left(\frac{1}{2} K_n\left(w^\star,\boldsymbol{t}\right) + V_n\left(w^\star,\boldsymbol{t}\right) + W_n\left(w^\star,\boldsymbol{t}\right)\right)\leq 0 \right)\;.
\end{multline*}
By Lemma \ref{lem:almost72LM}, the conclusion thus follows if
\begin{equation*}
% P \left( \min_{ \boldsymbol{t} \in \mathcal{C}_{\alpha,\gamma,n}' \left(\mathcal{I}\right) } 
% J_n \left( \overline{w}, \boldsymbol{t} \right) 
% - J_n \left( w^\star, \boldsymbol{t} \right) 
% + \frac{1}{2} K_n \left( w^\star , \boldsymbol{t} \right) \right) \right) \leq 0 \right ) & \longrightarrow_{n\rightarrow\infty} & 0
P \left( \min_{ \boldsymbol{t} \in \mathcal{C}_{\alpha,\gamma,n}' \left(\mathcal{I}\right) } 
\left(J_n \left( \overline{w}, \boldsymbol{t} \right) 
- J_n \left( w^\star, \boldsymbol{t} \right) 
+ \frac{1}{2} K_n \left( w^\star , \boldsymbol{t} \right)\right) \leq 0 \right ) 
 \longrightarrow 0\;, \textrm{ as } n\to\infty\;.
\end{equation*}
Since $\underset{\boldsymbol{t}\in \mathcal{C}_{\alpha,\gamma,n}'\left(\mathcal{I}\right)}{\min} K_n\left(w^\star,\boldsymbol{t}\right) \geq \left(1-\gamma\right)\Delta_{\boldsymbol{\tau}^\star}\alpha$ \parencite[Equation (65)]{LM}, 
$$P\left( \min_{\boldsymbol{t}\in \mathcal{C}_{\alpha,\gamma,n}'\left(\mathcal{I}\right)} \left( J_n\left(\overline{w},\boldsymbol{t}\right)-J_n\left(w^\star,\boldsymbol{t}\right)+\frac{1}{2} K_n\left(w^\star,\boldsymbol{t}\right)\right)\leq 0\right)$$
$$ \leq P\left(\min_{\boldsymbol{t}\in \mathcal{C}_{\alpha,\gamma,n}'\left(\mathcal{I}\right)} \left(J_n\left(\overline{w},\boldsymbol{t} \right)-J_n\left(w^\star,\boldsymbol{t}\right)\right) \leq \frac{1}{2} \left(\gamma-1\right)\Delta_{\boldsymbol{\tau}^\star}\alpha\right)\;, $$
 and we conclude by Lemma \ref{lem:BoundedUnifBound}.
\end{proof}

\begin{proof}[Proof of Lemma \ref{lem:rateT}]For notational simplicity, $\boldsymbol{\widehat{t}}_n(z, \overline{\Phi}_n)$ will be replaced by $\boldsymbol{\overline{t}}_n$ in this proof.
Since for any $\alpha>0$,
$$
P\left(\Vert  \boldsymbol{\overline{t}}_n - \boldsymbol{t}_n^\star\Vert_\infty< \alpha \underline{\lambda}^{-2}\right)
=P( \Vert\boldsymbol{\overline{t}}_n - \boldsymbol{t}_n^\star \Vert_\infty\leq n \gamma \Delta_{\boldsymbol{\tau}^\star} ) - P( \boldsymbol{\overline{t}}_n \in C_{\alpha , \gamma ,n })\;,
$$
it is enough, by Lemma \ref{lem:consistency}, to prove that
\begin{equation*}%\label{eq:C}
P\left(\boldsymbol{\overline{t}}_n \in \mathcal{C}_{\alpha,\gamma,n}\right) \longrightarrow 0\;,\; \textrm{as } n\to\infty\;,
\end{equation*}
for all $\alpha>0$ and $0<\gamma<1/2 $.
Since
$  \mathcal{C}_{\alpha,\gamma,n} = \underset{\mathcal{I}\subset\lbrace 1,\dots ,m\rbrace}{\bigcup} \mathcal{C}_{\alpha,\gamma,n}\cap \left\lbrace \boldsymbol{t}\in\mathcal{A}_{n,m}; \forall k \in \mathcal{I}, t_k\geq t_{n,k}^\star\right\rbrace $, we shall only study one set in the union without loss of generality and prove that
\begin{equation*}%\label{eq:C'}
P\left(\boldsymbol{\overline{t}}_n \in \mathcal{C}_{\alpha,\gamma,n}'\right) \longrightarrow 0\;,\; \textrm{as } n\to\infty\;,
\end{equation*}
where $\mathcal{C}_{\alpha,\gamma,n}'$ is defined in (\ref{eq:C'_alpha_gamma_n}). Since
$\mathcal{C}_{\alpha,\gamma,n}' = \underset{\mathcal{I}\subset\lbrace 1,\dots ,m\rbrace}{\bigcup} \mathcal{C}_{\alpha,\gamma,n}'\left(\mathcal{I}\right)$,
we shall only study one set in the union without loss of generality and prove that
\begin{equation*}%\label{eq:C'I}
P\left(\boldsymbol{\overline{t}}_n \in \mathcal{C}_{\alpha,\gamma,n}'\left(\mathcal{I}\right)\right) \longrightarrow 0\;,\; \textrm{as } n\to\infty\;.
\end{equation*}
Since 
$$ P\left(\boldsymbol{\overline{t}}_n \in \mathcal{C}_{\alpha,\gamma,n}'\left(\mathcal{I}\right)\right) \leq P\left(\min_{\boldsymbol{t} \in \mathcal{C}_{\alpha,\gamma,n}'\left(\mathcal{I}\right)} J_n\left(\overline{w},\boldsymbol{t} \right)\leq 0\right)\;,$$
the proof is complete by Lemma \ref{lem:almost72LM2}.

\end{proof}

\begin{proof}[Proof of Proposition \ref{Prop:Segment}]For notational simplicity, $\boldsymbol{\widehat{\delta}}_n(z, \overline{\Phi}_n)$ will be replaced by $\boldsymbol{\overline{\delta}}_n$ in this proof.
By Lemma \ref{lem:rateT}, the last result to show is
\begin{equation*}
\Vert \boldsymbol{\overline{\delta}_n}-\boldsymbol{\delta}^\star\Vert = O_P\left(n^{-1/2}\right)\;,
\end{equation*}
that is, for all $k$,
$
\overline{\delta}_{n,k} - \delta_k^\star = O_P\left(n^{-1/2}\right).
$
By \eqref{eq:decor} and \eqref{eq:overline_x},
\begin{eqnarray*}
\overline{\delta}_{n,k} & = & \frac{1}{\overline{t}_{n,k+1}-\overline{t}_{n,k}} \sum_{i=\overline{t}_{n,k}+1}^{\overline{t}_{n,k+1}}\overline{w}_i
  =  \frac{1}{n\left(\overline{\tau}_{n,k+1}-\overline{\tau}_{n,k}\right)}\left( \sum_{i=\overline{t}_{n,k}+1}^{\overline{t}_{n,k+1}}w_i^\star + \sum_{r=1}^p \left( \phi_r^\star - \overline{\phi}_{r,n}\right) \sum_{i=\overline{t}_{n,k}+1}^{\overline{t}_{n,k+1}} z_{i-r} \right)\;.
\end{eqnarray*}
By the Cauchy-Schwarz inequality,
\begin{eqnarray*}
\left\vert \sum_{i=\overline{t}_{n,k}+1}^{\overline{t}_{n,k+1}}z_{i-r} \right\vert & \leq & \left(\overline{t}_{n,k+1}-\overline{t}_{n,k}\right)^{1/2}
\left(z_{\overline{t}_{n,k}+1-r}^2+ \dots +z_{\overline{t}_{n,k+1}-r}^2\right)^{1/2} 
  \leq  n^{1/2} \left\Vert Bz \right\Vert
  =  O_P\left(n\right)\;,
\end{eqnarray*}
where the last equality comes from Lemma \ref{lem:rateXY}. Hence by \eqref{eq:hypRhoRate} and Lemma \ref{lem:rateT},
\begin{eqnarray*}
\overline{\delta}_{n,k} & = & \frac{1}{n\left(\overline{\tau}_{n,k+1}-\overline{\tau}_{n,k}\right)} \sum_{i=\overline{t}_{n,k}+1}^{\overline{t}_{n,k+1}}w_i^\star + O_P\left(n^{-1/2}\right)\\
 & = & \frac{1}{n\left(\overline{\tau}_{n,k+1}-\overline{\tau}_{n,k}\right)} \left(\sum_{i=\overline{t}_{n,k}+1}^{\overline{t}_{n,k+1}}\mathbb{E} w_i^\star + \sum_{i=\overline{t}_{n,k}+1}^{\overline{t}_{n,k+1}} \epsilon_i\right) + O_P\left(n^{-1/2}\right),
\end{eqnarray*}
where the last equality comes from (\ref{eq:modele_matriciel}) and (\ref{eq:decor}).

Let us now prove that 
\begin{equation}\label{eq:clt_aleatoire}
\frac{1}{n\left(\overline{\tau}_{n,k+1}-\overline{\tau}_{n,k}\right)} \sum_{i=\overline{t}_{n,k}+1}^{\overline{t}_{n,k+1}} \epsilon_i = O_P\left(n^{-1/2}\right)\;.
\end{equation}
By Lemma \ref{lem:consistency}, $n^{-1}\left(\overline{\tau}_{n,k+1}-\overline{\tau}_{n,k}\right)^{-1}=O_P(n^{-1})$. Moreover,
\begin{equation}\label{eq:eps_decomp}
\sum_{i=\overline{t}_{n,k}+1}^{\overline{t}_{n,k+1}} \epsilon_i = \sum_{i=t_{n,k}^\star+1}^{t_{n,k+1}^\star} \epsilon_i \pm \sum_{i=\overline{t}_{n,k}+1}^{t_{n,k}^\star} \epsilon_i \pm \sum_{i=t_{n,k+1}^\star}^{\overline{t}_{n,k+1}+1} \epsilon_i\;.
\end{equation}
By the Central limit theorem, the first term in the right-hand side of (\ref{eq:eps_decomp}) is $O_P(n^{1/2})$. By using the Cauchy-Schwarz inequality, we get that 
the second term of (\ref{eq:eps_decomp}) satisfies:
$|\sum_{i=\overline{t}_{n,k}+1}^{t_{n,k}^\star} \epsilon_i|\leq |t_{n,k}^\star-\overline{t}_{n,k}|^{1/2} \left(\sum_{i=1}^n  \epsilon_i^2\right)^{1/2}=O_P(1) O_P(n^{1/2})=O_P(n^{1/2})$, by Lemma 
\ref{lem:rateT}. The same holds for the last term in the right-hand side of \eqref{eq:eps_decomp}, which gives \eqref{eq:clt_aleatoire}.

Hence,
\begin{eqnarray*}
\overline{\delta}_{n,k} - \delta_k^\star & = & \frac{1}{n\left(\overline{\tau}_{n,k+1}-\overline{\tau}_{n,k}\right)} \sum_{i=\overline{t}_{n,k}+1}^{\overline{t}_{n,k+1}}\left(\mathbb{E} w_i^\star - \delta_k^\star\right) + O_P\left(n^{-1/2}\right)\\
 & = &  \frac{1}{n\left(\overline{\tau}_{n,k+1}-\overline{\tau}_{n,k}\right)} \sum_{i\in\left\lbrace\overline{t}_{n,k}+1,\dots ,\overline{t}_{n,k+1}\right\rbrace \setminus \left\lbrace t_{n,k}^\star+1,\dots ,t_{n,k+1}^\star\right\rbrace}\left(\mathbb{E} w_i^\star - \delta_k^\star\right) + O_P\left(n^{-1/2}\right)\;,
\end{eqnarray*}
and then
\begin{eqnarray*}
\left\vert \overline{\delta}_{n,k} - \delta_k^\star \right\vert & \leq & \frac{1}{n\left(\overline{\tau}_{n,k+1}-\overline{\tau}_{n,k}\right)} \sharp\left\lbrace\overline{t}_{n,k}+1,\dots ,\overline{t}_{n,k+1}\right\rbrace \setminus \left\lbrace t_{n,k}^\star+1,\dots ,t_{n,k+1}^\star\right\rbrace \max_{l= 0,\dots,m}\left\vert \delta_l^\star - \delta_k^\star\right\vert \\
 & + & O_P\left(n^{-1/2}\right)\;.
\end{eqnarray*}

We conclude by using Lemma \ref{lem:rateT} to get $\sharp\left\lbrace\overline{t}_{n,k}+1,\dots ,\overline{t}_{n,k+1}\right\rbrace \setminus \left\lbrace t_{n,k}^\star+1,\dots ,t_{n,k+1}^\star\right\rbrace = O_P\left(1\right)$ and Lemma \ref{lem:consistency} to get $\left(\overline{\tau}_{n,k+1}-\overline{\tau}_{n,k}\right)^{-1} = O_P\left(1\right)$.
\end{proof}

\subsection{Proof of Proposition \ref{Prop:Segment2}}\label{subsec:prop:Segment2}

The connection between Models~\eqref{eq:modele_new} and~\eqref{eq:bkw} is made by the following lemmas.

\begin{lemma} \label{Lem:YZ}
 Let $(y_0, \dots y_n)$ be defined by \eqref{eq:modele_new} and let
 \begin{eqnarray}
 v^\star_i & = & y_i - \sum_{r=1}^p \phi_r^\star y_{i-1}\label{eq:v_star},\\
 \Delta^\star_i & = & \begin{cases}
%\left\lbrace
-\left(\mu^\star_k  - \mu^\star_{k-1}\right)\sum_{s=r}^p\phi_s^\star \textit{ if } i = t_{n,k}^\star+r \textit{ and } 1\leq r \leq p\\
0, \textit{ otherwise, }
%\right.
\end{cases} \label{eq:delta_star}
 \end{eqnarray} where the $\mu_k^\star$'s are defined in \eqref{eq:modele_new}, then the process 
\begin{equation}\label{eq:vw_star}
 w^\star_i = v^\star_i + \Delta^\star_i
\end{equation}
equals $z_i - \sum_{r=1}^p z_{i-r}$ where $(z_{1-p}, \dots , z_n)$ verify \eqref{eq:bkw}. Such a process $(z_{1-p}, \dots , z_n)$ can be constructed recursively as

\begin{equation}\label{eq:z_rec}
\begin{cases}
%\left\lbrace
z_i & =  y_i \textit{ for } 1-p\leq i\leq 0\\
z_i & =  w^\star_i + \sum_{r=1}^p \phi_r^\star z_{i-r} \textit{ for } i>0.
%\right.
\end{cases}
\end{equation}
\end{lemma}

\begin{lemma}\label{Lem:YZbar}
 Let $(y_{1-p}, \dots , y_n)$ be defined by \eqref{eq:modele_new} and let $z$ be defined by (\ref{eq:v_star}-- \ref{eq:z_rec}). Then
\begin{equation}\label{eq:vw}
\overline{w}_i = \overline{v}_i + \overline{\Delta}_i
\end{equation}
where
\begin{eqnarray}
\overline{v}_i & = & y_i - \sum_{r=1}^p\overline{\phi}_{r,n} y_{i-r}\label{eq:v_bar}\\
\overline{w}_i & = & z_i - \sum_{r=1}^p\overline{\phi}_{r,n} z_{i-r}\label{eq:w_bar}\\
\overline{\Delta}_i & = & \Delta^\star_i + \sum_{r=1}^p\left(\phi_r^\star - \overline{\phi}_{r,n}\right)\left(z_{i-r}-y_{i-r}\right)\; .\label{eq:Delta_bar}
\end{eqnarray}
\end{lemma}

\begin{lemma} \label{Lem:Delta_order}
 Let $\overline{\Delta}=(\overline{\Delta}_i)_{0\leq i\leq n}$ as defined in \eqref{eq:Delta_bar}. 
Then $\left\Vert\overline{\Delta}\right\Vert = O_P\left(1\right)$.
\end{lemma}

\begin{proof}[Proof of Lemma \ref{Lem:YZ}.]
Let $z$ being defined by \eqref{eq:z_rec}. Using \eqref{eq:vw_star}, we get, for all $0\leq k \leq m , t_{n,k}^\star<i\leq t_{n,k+1}^\star$
\begin{multline*}
\left(z_i - \mu_k^\star \right) - \sum_{r=1}^p\phi_r^\star \left(z_{i-r} - \mu_k^\star\right) = \left(y_i - \mu_k^\star\right) - \sum_{r=1}^p\phi_r^\star \left(y_{i-r} - \mu_k^\star\right) + \Delta_i^\star \\
 = \left(y_i - \mu_k^\star\right) - \sum_{r=1}^{p} \phi_r^\star \left(y_{i-1} - (\mu_{k-1}^\star \mathbf{1}_{r\geq i-t_{n,k}^\star} + \mu_k^\star \mathbf{1}_{r< i-t_{n,k}^\star})\right)
%\begin{cases}
%\left\lbrace
%\left(y_i - \mu_k^\star\right) - \sum_{s=1}^{r-1} \phi_s^\star \left(y_{i-1} - \mu_{k-1}^\star\right) \textit{ if } i = t_{n,k}^\star+1\\
%\left(y_i - \mu_k^\star\right) - \rho^\star \left(y_{i-1} - \mu_k^\star\right) \textit{ otherwise.}
%\right.
%\end{cases}
\end{multline*}
This expression equals $\left(y_i - \PE \left(y_i\right)\right) - \sum_{r=1}^p\phi_r^\star \left(y_{i-r} - \PE\left(y_{i-r}\right)\right) = \eta_i - \sum_{r=1}^p \phi_r^\star \eta_{i-r} = \epsilon_i$ by \eqref{eq:modele_new} and \eqref{eq:arp}. Then $z$ satisfies \eqref{eq:bkw}.
\end{proof}
The proof of Lemma \ref{Lem:YZbar} is straightforward.
\begin{proof}[Proof of Lemma \ref{Lem:Delta_order}]
\eqref{eq:Delta_bar} can be written as
$$
\overline{\Delta} = \Delta^\star + \sum_{r=1}^p\left(\phi_r^\star - \overline{\phi}_{r,n}\right)\left(B^r y-B^r z\right)
$$
where $\Delta^\star=\left(\Delta_i^\star\right)_{1\leq i\leq n}$, $B^r y = \left(y_{i-r}\right)_{1\leq i\leq n}$  and $B^r z$ is defined in \eqref{eq:YXE}. By the triangle inequality,
\begin{equation}\label{eq:triangular_Delta_bar}
\left\Vert\overline{\Delta}\right\Vert \leq \left\Vert\Delta^\star\right\Vert + \sum_{r=1}^p \left\vert\phi_r^\star - \overline{\phi}_{r,n} \right\vert \left(\left\Vert B^r y\right\Vert+\left\Vert B^r z\right\Vert\right).
\end{equation}
Since $\left\Vert\Delta^\star\right\Vert$ is constant in $n$ it is bounded.
The conclusion follows from \eqref{eq:triangular_Delta_bar}, \eqref{eq:hypRhoRate} and Lemma \ref{lem:rateXY}.
\end{proof}

\begin{proof}[Proof of Proposition \ref{Prop:Segment2}]
Let $y$, $z$, $\overline{v}$, $\overline{w}$ and $\overline{\Delta}$ be defined in Lemma \ref{Lem:YZbar}.

Using \eqref{eq:Jnm} and Lemma \ref{Lem:YZbar}, we get
\begin{equation*}
J_n\left(\overline{v},\boldsymbol{t}\right) = J_n\left(\overline{w},\boldsymbol{t}\right) + J_n\left(\overline{\Delta},\boldsymbol{t}\right) - \frac{2}{n}\left(\left\langle \pi_{E_{\boldsymbol{t}_n^\star}}\left(\overline{w}\right),\pi_{E_{\boldsymbol{t}_n^\star}}\left(\overline{\Delta}\right)\right\rangle - \left\langle \pi_{E_{\boldsymbol{t}}}\left(\overline{w}\right),\pi_{E_{\boldsymbol{t}}}\left(\overline{\Delta}\right)\right\rangle\right).
\end{equation*}
By the Cauchy-Schwarz inequality and the $1$-Lipschitz property of projections, we have
\begin{eqnarray*}%\label{eq:CSLipschitz}
\left\vert J_n\left(\overline{\Delta},\boldsymbol{t} \right) \right\vert & \leq & 2 \Vert \overline{\Delta} \Vert^2 ,\\%\label{eq:CSLipschitz1}, \\
\left\vert \left\langle \pi_{E_{\boldsymbol{t}_n^\star}}\left(\overline{w}\right),\pi_{E_{\boldsymbol{t}_n^\star}}\left(\overline{\Delta}\right)\right\rangle - \left\langle \pi_{E_{\boldsymbol{t}}}\left(\overline{w}\right),\pi_{E_{\boldsymbol{t}}}\left(\overline{\Delta}\right)\right\rangle \right\vert & \leq & 2 \Vert \overline{\Delta} \Vert \Vert \overline{w} \Vert. % \label{eq:CSLipschitz2}
\end{eqnarray*}
Note that $\overline{w} = z - \sum_{r=1}^p \overline{\phi}_{r,n} B^r z$ thus by the triangle inequality

\begin{equation*}%\label{eq:triangular}
\Vert \overline{w}\Vert \leq \Vert z \Vert + \sum_{r=1}^p \vert \overline{\phi}_{r,n} \vert \Vert B^r z \Vert \; .
\end{equation*}

Since $\vert \overline{\phi}_{r,n} \vert = O_P\left(1\right)$ for all $1\leq r\leq p$, we deduce from Lemma \ref{lem:rateXY} that $\Vert \overline{w}\Vert=O_P \left(n^{1/2}\right)$. Since, by Lemma \ref{Lem:Delta_order}, $\Vert \overline{\Delta} \Vert = O_P\left(1\right)$, we
obtain that

\begin{equation}\label{eq:controleunif}
\sup_{\boldsymbol{t}} \left\lbrace J_n\left(\overline{\Delta},\boldsymbol{t}\right) - \frac{2}{n}\left(\left\langle \pi_{E_{\boldsymbol{t}_n^\star}}\left(\overline{w}\right),\pi_{E_{\boldsymbol{t}_n^\star}}\left(\overline{\Delta}\right)\right\rangle - \left\langle \pi_{E_{\boldsymbol{t}}}\left(\overline{w}\right),\pi_{E_{\boldsymbol{t}}}\left(\overline{\Delta}\right)\right\rangle\right) \right\rbrace =O_P\left(n^{-1/2}\right).
\end{equation}
For $0<\alpha<\Delta_{\boldsymbol{\tau}^\star}$, using \eqref{eq:Jn_decomp} and \eqref{eq:Cn_alpha}, we get:
\begin{eqnarray*}
P\left(\left\Vert \boldsymbol{\overline{t}}_n - \boldsymbol{t}^\star \right\Vert_{\infty} \geq \alpha\right)  & \leq & P \left( \min_{\boldsymbol{t}\in\mathcal{C}_{n,\alpha}} J_n \left(\overline{v}, \boldsymbol{t} \right) \leq 0\right)\\
  & \leq & P \left( \min_{\boldsymbol{t} \in\mathcal{C}_{n,\alpha}} \left\lbrace J_n\left(\overline{w},\boldsymbol{t}\right) + J_n\left(\overline{\Delta},\boldsymbol{t}\right)  \right.\right. \\
  & & \ \ - \left.\left. \frac{2}{n}\left(\left\langle \pi_{E_{\boldsymbol{t}_n^\star}}\left(\overline{w}\right),\pi_{E_{\boldsymbol{t}_n^\star}}\left(\overline{\Delta}\right)\right\rangle - \left\langle \pi_{E_{\boldsymbol{t}}}\left(\overline{w}\right),\pi_{E_{\boldsymbol{t}}}\left(\overline{\Delta}\right)\right\rangle\right)\right\rbrace \leq 0 \right)\\
 & \leq & P \left( \min_{\boldsymbol{t}\in\mathcal{C}_{n,\alpha}} \left\lbrace K_n\left(\overline{w},\boldsymbol{t}\right) + V_n\left(\overline{w},\boldsymbol{t}\right) + W_n\left(\overline{w},\boldsymbol{t}\right)+ J_n\left(\overline{\Delta},\boldsymbol{t}\right) \right. \right. \\
  & & \ \ - \left. \left. \frac{2}{n}\left(\left\langle \pi_{E_{\boldsymbol{t}_n^\star}}\left(\overline{w}\right),\pi_{E_{\boldsymbol{t}_n^\star}}\left(\overline{\Delta}\right)\right\rangle - \left\langle \pi_{E_{\boldsymbol{t}}}\left(\overline{w}\right),\pi_{E_{\boldsymbol{t}}}\left(\overline{\Delta}\right)\right\rangle\right)\right\rbrace \leq 0 \right)\\
  & \leq & P \left( \min_{\boldsymbol{t}\in\mathcal{C}_{n,\alpha}} \left\lbrace \frac{1}{2}K_n\left(\overline{w},\boldsymbol{t}\right) + V_n\left(\overline{w},\boldsymbol{t}\right) + W_n\left(\overline{w},\boldsymbol{t}\right)\right\rbrace \leq 0 \right)\\
   & & + P \left( \min_{\boldsymbol{t}\in\mathcal{C}_{n,\alpha}} \left\lbrace \frac{1}{2}K_n\left(\overline{w},\boldsymbol{t}\right) + J_n\left(\overline{\Delta},\boldsymbol{t}\right) \right. \right. \\
   & & \ \ - \left. \left. \frac{2}{n}\left(\left\langle \pi_{E_{\boldsymbol{t}_n^\star}}\left(\overline{w}\right),\pi_{E_{\boldsymbol{t}_n^\star}}\left(\overline{\Delta}\right)\right\rangle - \left\langle \pi_{E_{\boldsymbol{t}}}\left(\overline{w}\right),\pi_{E_{\boldsymbol{t}}}\left(\overline{\Delta}\right)\right\rangle\right)\right\rbrace \leq 0 \right).
\end{eqnarray*}
Following the proof of Lemma \ref{lem:consistency}, one can prove that $$P \left( \underset{\boldsymbol{t}\in\mathcal{C}_{n,\alpha}}{\min} \left\lbrace\frac{1}{2}K_n\left(\overline{w},\boldsymbol{t}\right) + V_n\left(\overline{w},\boldsymbol{t}\right) + W_n\left(\overline{w},\boldsymbol{t}\right)\right\rbrace \leq 0\right) \underset{n\rightarrow\infty}{\longrightarrow} 0 \; .$$
Using \eqref{eq:LMbounds}, we get that
\begin{eqnarray*}
P \left( \min_{\boldsymbol{t}\in\mathcal{C}_{n,\alpha}} \left\lbrace\frac{1}{2}K_n\left(\overline{w},\boldsymbol{t}\right) +  J_n\left(\overline{\Delta},\boldsymbol{t}\right) - \frac{2}{n}\left(\left\langle \pi_{E_{\boldsymbol{t}_n^\star}}\left(\overline{w}\right),\pi_{E_{\boldsymbol{t}_n^\star}}\left(\overline{\Delta}\right)\right\rangle - \left\langle \pi_{E_{\boldsymbol{t}}}\left(\overline{w}\right),\pi_{E_{\boldsymbol{t}}}\left(\overline{\Delta}\right)\right\rangle\right)\right\rbrace \leq 0\right) & & \\
 \leq P \left( \frac{1}{2}\underline{\lambda}^2 \alpha + \min_{\boldsymbol{t}\in\mathcal{C}_{n,\alpha}}  \left\{ J_n\left(\overline{\Delta},\boldsymbol{t}\right) - \frac{2}{n}\left(\left\langle \pi_{E_{\boldsymbol{t}_n^\star}}\left(\overline{w}\right),\pi_{E_{\boldsymbol{t}_n^\star}}\left(\overline{\Delta}\right)\right\rangle - \left\langle \pi_{E_{\boldsymbol{t}}}\left(\overline{w}\right),\pi_{E_{\boldsymbol{t}}}\left(\overline{\Delta}\right)\right\rangle\right)\right\} \leq 0\right) & & \\
\end{eqnarray*}
which goes to zero when $n$ goes to infinity by \eqref{eq:controleunif}.

Then Lemma \ref{lem:consistency} still holds if $y$ is defined by \eqref{eq:modele_new}.
To show the rate of convergence, we use the same decomposition. As in the proof of Lemma \ref{lem:rateT}, $P\left(\underset{\boldsymbol{t} \in \mathcal{C}_{\alpha,\gamma,n}'\left(\mathcal{I}\right)}{\min} J_n\left(\overline{v},\boldsymbol{t}\right)\leq 0\right)\underset{n\rightarrow \infty}{\longrightarrow} 0$ for all $\alpha>0$ and $0<\gamma <1/2$ is a sufficient condition 
for proving that $P\left(\boldsymbol{\widehat{t}}_n(y,\overline{\rho}_n)\in \mathcal{C}_{\alpha,\gamma,n}\right) \longrightarrow_{n\rightarrow\infty} 0$, which allows us to conclude on the rate of convergence of the estimated change-points. Note that
\begin{eqnarray*}
P\left(\min_{\boldsymbol{t} \in \mathcal{C}_{ \alpha, \gamma, n}'\left(\mathcal{I}\right)} J_n\left(\overline{v},\boldsymbol{t}\right) \leq 0\right)  & \leq & P \left( \min_{\boldsymbol{t} \in \mathcal{C}_{\alpha,\gamma,n}'} 
\left\lbrace\frac{1}{2}K_n\left( \overline{w}, \boldsymbol{t} \right) + V_n \left( \overline{w}, \boldsymbol{t}\right) + W_n \left( \overline{w}, \boldsymbol{t} \right)\right\rbrace \leq 0\right)\\
   & + & P \left( \frac{1}{2}\underline{\lambda}^2 \alpha + J_n\left(\overline{\Delta},\boldsymbol{t}\right) \right. \\
   & - & \left. \frac{2}{n}\left(\left\langle \pi_{E_{\boldsymbol{t}_n^\star}}\left(\overline{w}\right),\pi_{E_{\boldsymbol{t}_n^\star}}\left(\overline{\Delta}\right)\right\rangle - \left\langle \pi_{E_{\boldsymbol{t}}}\left(\overline{w}\right),\pi_{E_{\boldsymbol{t}}}\left(\overline{\Delta}\right)\right\rangle\right) \leq 0 \right).
\end{eqnarray*}
In the latter equation, the second term of the right-hand side goes to zero as $n$ goes to infinity by \eqref{eq:controleunif}.
The first term of the right-hand side goes to zero when $n$ goes to infinity by following the same line of reasoning as the one of Lemma \ref{lem:almost72LM2}. This concludes the proof of Proposition \ref{Prop:Segment2}.
\end{proof}

%%% Local Variables:
%%% mode: latex
%%% TeX-master: "Cha13.tex"
%%% End:

\subsection{Proof of Proposition \ref{ar1:Prop:SelBeta}}\label{ar1:subsec:bicbardet}
We shall used in this section the notations introduced in Sections \ref{ar1:subsec:prop:Segment} and \ref{ar1:subsec:beta}.
 The result derives directly from Lemmas \ref{ar1:Lem:infSelBeta} and \ref{ar1:Lem:supSelBeta}.
 
\begin{lemma}\label{ar1:Lem:infSelBeta}
Under the assumptions of Proposition \ref{ar1:Prop:SelBeta}, $P\left(\widehat{m}=m\right)\underset{n\rightarrow\infty}{\longrightarrow} 0$ if $m<m^{\star}$.
\end{lemma}
\begin{lemma}\label{ar1:Lem:supSelBeta}
Under the assumptions of Proposition \ref{ar1:Prop:SelBeta}, $P\left(\widehat{m}=m\right)\underset{n\rightarrow\infty}{\longrightarrow} 0$ if $m>m^{\star}$.
\end{lemma}

\begin{proof}[Proof of Lemma \ref{ar1:Lem:infSelBeta}]
If $\widehat{m}=m<m^{\star}$, then
\begin{equation*}
\frac1n SS_m(z, \overline{\rho}_n) + \beta_n m \leq \frac1n SS_{m^{\star}}(z, \overline{\rho}_n) + \beta_n m^{\star} \; ,
\end{equation*}
where $SS_m$ is defined in \eqref{ar1:Eq:SSm}. In particular, there exists $\boldsymbol{t}\in \mathcal{A}_{n,m}$ such that
\begin{equation*}
\frac1n \underset{\boldsymbol{\delta}}{\min} SS_m(z, \overline{\rho}_n, \boldsymbol{\delta}, \boldsymbol{t}) + \beta_n m \leq \frac1n \underset{\boldsymbol{\delta}}{\min} SS_m(z, \overline{\rho}_n, \boldsymbol{\delta}, \boldsymbol{t}_n^{\star}) + \beta_n m^{\star} \; .
\end{equation*}
From \eqref{ar1:eq:Jnm}, we get
\begin{equation*}
J_n \left(\overline{w},\boldsymbol{t}\right) \leq \beta_n\left(m^{\star} - m\right) \; .
\end{equation*}
Since $\left(\beta_n\right)$ converges to zero, for any $\varepsilon>0$, $\beta_n\left(m^{\star} - m\right) \leq \varepsilon$ for a large
enough $n$, and so
\begin{equation*}
J_n \left(\overline{w},\boldsymbol{t}\right) \leq \varepsilon \; .
\end{equation*}
One can check that there exist $0<\nu<\Delta_{\boldsymbol{\tau}^{\star}}$ such that, for a large enough $n$, there exists $\boldsymbol{t}'\in \mathcal{C}_{n,m^{\star},\nu}$ such that $E_{\boldsymbol{t}} \subset E_{\boldsymbol{t}'}$ (that is the change-points of $\boldsymbol{t}$ are change-points of $\boldsymbol{t}'$) for all $\boldsymbol{t}\in \mathcal{A}_{n,m}$, where $\mathcal{C}_{n,m^{\star},\nu}$ is defined in \eqref{ar1:eq:Cn_alpha}. From \eqref{ar1:eq:Jnm} and $E_{\boldsymbol{t}} \subset E_{\boldsymbol{t}'}$, we get $J_n \left(\overline{w},\boldsymbol{t}'\right) \leq J_n \left(\overline{w},\boldsymbol{t}\right)$. Then, the following inequality holds for all $\varepsilon>0$ and any large enough $n$:
\begin{equation}\label{ar1:eq:ineq_inf_beta}
P\left(\widehat{m}=m\right) \leq P\left(\exists \boldsymbol{t}'\in \mathcal{C}_{n,m^{\star},\nu} , J_n \left(\overline{w},\boldsymbol{t}'\right) \leq \varepsilon\right) \; .
\end{equation}
We then follow the steps of \eqref{ar1:eq:ineq_alpha}, $-\nu\underline{\lambda}^2$ being replaced by $\varepsilon-\nu\underline{\lambda}^2$. The convergence of $P\left(\exists \boldsymbol{t}'\in \mathcal{C}_{n,m^{\star},\nu} , J_n \left(\overline{w},\boldsymbol{t}'\right) \leq \varepsilon\right)$ to zero holds with $\varepsilon < \nu\underline{\lambda}^2$. We can conclude with \eqref{ar1:eq:ineq_inf_beta}.
\end{proof}
\begin{proof}[Proof of Lemma \ref{ar1:Lem:supSelBeta}]
Following the proof of Lemma \ref{ar1:Lem:infSelBeta}, if $\widehat{m}=m>m^{\star}$, there exists $\boldsymbol{t}\in\mathcal{A}_{n,m}$ such that $J_n \left(\overline{w},\boldsymbol{t}\right) \leq \beta_n\left(m^{\star} - m\right)$ and then $ J_n \left(\overline{w},\boldsymbol{t}\right) + \beta_n \leq 0 $ since $m>m^{\star}$. Then
\begin{equation}\label{ar1:eq:ineq_sup_beta}
P\left(\widehat{m}=m\right) \leq P\left(\exists \boldsymbol{t}\in \mathcal{A}_{n,m} , J_n \left(\overline{w},\boldsymbol{t}\right) + \beta_n \leq 0\right) \; .
\end{equation}
Adding the change-points of $\boldsymbol{t}_n^{\star}$ to those of such a $\boldsymbol{t}$, one can get $t'\in\mathcal{A}_{n,m'}$ with $m^{\star}<m\leq m' \leq m+m^{\star}$ such that $E_{\boldsymbol{t}}\cup E_{\boldsymbol{t}_n^{\star}}\subset E_{\boldsymbol{t}'}$, provided that $\left(m+m^{\star}\right)\left\lceil\Delta_n\right\rceil\leq n$, where $\lceil\cdot \rceil$ is the ceiling function, this condition being fulfilled for any sufficiently large $n$ under the assumptions of Proposition \ref{ar1:Prop:SelBeta} since $n^{-1}\Delta_n$ converges to zero. Since $E_{\boldsymbol{t}}\subset E_{\boldsymbol{t}'}$, we derive $J_n \left(\overline{w},\boldsymbol{t}'\right)+ \beta_n \leq J_n \left(\overline{w},\boldsymbol{t}\right) + \beta_n$ from \eqref{ar1:eq:Jnm}. Then, from \eqref{ar1:eq:ineq_sup_beta}, we get
\begin{equation}\label{ar1:eq:sublemma_sup_beta}
\forall m' > m^{\star} , P\left(\exists \boldsymbol{t}'\in \mathcal{A}_{n,m'} , E_{\boldsymbol{t}_n^{\star}}\subset E_{\boldsymbol{t}'},  J_n \left(\overline{w},\boldsymbol{t}'\right)+ \beta_n \leq 0\right) \underset{n\rightarrow\infty}{\longrightarrow} 0
\end{equation}
is a sufficient condition to prove the lemma. Let us prove \eqref{ar1:eq:sublemma_sup_beta}. Let $m'>m^{\star}$ and such a $\boldsymbol{t}'$. We compare $J_n \left(\overline{w},\boldsymbol{t}'\right)$ to $J_n \left(w^{\star},\boldsymbol{t}'\right)$. Since $\mathbb{E}w^{\star}\in E_{\boldsymbol{t}_n^{\star}}\subset E_{\boldsymbol{t}'}$, $K_n \left(w^{\star} , \boldsymbol{t}'\right) = 0$ by \eqref{ar1:eq:Kn}. By~\eqref{ar1:eq:Wn} and $\mathbb{E}w^{\star}\in E_{\boldsymbol{t}_n^{\star}}\subset E_{\boldsymbol{t}'}$,
\begin{eqnarray*}
W_n\left(w^{\star},\boldsymbol{t}'\right) & = & \frac{2}{n}\left( \left\langle \pi_{E_{\boldsymbol{t}_n^{\star}}} \left( w^{\star}-\mathbb{E}w^{\star}\right), \pi_{E_{\boldsymbol{t}_n^{\star}}} \left( \mathbb{E}w^{\star} \right)\right\rangle - \left\langle \pi_{E_{\boldsymbol{t}'}} \left( w^{\star}-\mathbb{E}w^{\star}\right), \pi_{E_{\boldsymbol{t}'}} \left( \mathbb{E}w^{\star} \right)\right\rangle  \right)\\
 & = & \frac{2}{n}\left\langle \pi_{E_{\boldsymbol{t}_n^{\star}}} \left( w^{\star}-\mathbb{E}w^{\star}\right) - \pi_{E_{\boldsymbol{t}'}} \left( w^{\star}-\mathbb{E}w^{\star}\right), \pi_{E_{\boldsymbol{t}_n^{\star}}} \left( \mathbb{E}w^{\star} \right)\right\rangle \\
  & = & - \frac{2}{n}\left\langle \pi_{E_{\boldsymbol{t}_n^{\star}}^\bot} \pi_{E_{\boldsymbol{t}'}} \left( w^{\star}-\mathbb{E}w^{\star}\right), \pi_{E_{\boldsymbol{t}_n^{\star}}} \left( \mathbb{E}w^{\star} \right)\right\rangle \\
   & = & 0 \; ,
\end{eqnarray*}
where $E^\bot$ is the (Euclidian) orthogonal complement of the vector subspace $E$. Then $J_n \left(w^{\star},\boldsymbol{t}'\right) = V_n \left(w^{\star},\boldsymbol{t}'\right)$ and
\begin{equation}\label{ar1:eq:decomp_sup_beta}
J_n \left(\overline{w},\boldsymbol{t}'\right) = V_n \left(w^{\star},\boldsymbol{t}'\right) + \left(J_n \left(\overline{w},\boldsymbol{t}'\right) - J_n \left(w^{\star},\boldsymbol{t}'\right)\right) \; .
\end{equation}
Using \eqref{ar1:eq:LMboundV}, $V_n\left(w^{\star},\boldsymbol{t}\right)  \geq  -\frac{2\left(m'+1\right)}{n\Delta_n}M_n$, where
\begin{eqnarray*}
M_n & = & M_{n,1} + M_{n,2}\;,\\
 M_{n,1} & = & \max_{1\leq s\leq n} \left(\sum_{i=1}^s \epsilon_i\right)^2\;, \\
 M_{n,2} & = &  \max_{1\leq s\leq n} \left(\sum_{i=n-s}^{n} \epsilon_i\right)^2\;.
\end{eqnarray*}
 We define $D_n = \underset{\boldsymbol{t}' \in\mathcal{A}_{n,m'}}{\sup} \left| J_n \left(\overline{w},\boldsymbol{t}'\right) - J_n \left(w^{\star},\boldsymbol{t}'\right) \right|$. Then, using \eqref{ar1:eq:decomp_sup_beta},
\begin{equation*}
J_n \left(\overline{w},\boldsymbol{t}'\right) \geq -\frac{2\left(m+1\right)}{n\Delta_n}M_n - D_n \; ,
\end{equation*}
which implies
\begin{eqnarray*}
P\left(\exists \boldsymbol{t}'\in \mathcal{A}_{n,m'} , E_{\boldsymbol{t}_n^{\star}}\subset E_{\boldsymbol{t}'},  J_n \left(\overline{w},\boldsymbol{t}'\right)+ \beta_n \leq 0\right) & \leq & P\left( -\frac{2\left(m'+1\right)}{n\Delta_n}M_n - D_n + \beta_n \leq 0\right)\\
 & \leq & P\left( \frac{2\left(m'+1\right)}{n\Delta_n}M_n \geq \frac{\beta_n}{2} \right) + P\left(  D_n \geq \frac{\beta_n}{2} \right) \; .
\end{eqnarray*}
By Lemma \ref{ar1:lem:BoundedUnifBound}, $D_n = O_P \left(n^{-1/2}\right)$ and then $P\left(  D_n \geq \frac{\beta_n}{2} \right)$ tends to zero as $n$ tends to infinity since $n^{1/2}\beta_n\underset{n\rightarrow\infty}{\longrightarrow} + \infty $. Let us now prove that $P\left( \frac{2\left(m+1\right)}{n\Delta_n}M_n \geq \frac{\beta_n}{2} \right)$ tends to zero as $n$ tends to infinty, which concludes the proof. Note that
\begin{equation*}
P\left( \frac{2\left(m'+1\right)}{n\Delta_n}M_n \geq \frac{\beta_n}{2} \right) \leq P\left( M_{n,1} \geq \frac{n\Delta_n \beta_n}{8\left(m'+1\right)} \right) + P\left( M_{n,2} \geq \frac{n\Delta_n \beta_n}{8\left(m'+1\right)} \right) \; .
\end{equation*}
We prove the convergence for each term in the right-hand side of the above equation. We shall prove it for the first term in the right-hand side since the arguments for the other term are the same.  From  Kolmogorov's maximal inequality \parencite[see for example][Theorem 2.5.2.]{durrett2010probability}\footnote{See Theorem~\ref{th:kolmogorov} of this document.}, since $\left(\epsilon_i\right)_{i\geq 0}$ is a sequence of independent rv's with zero-mean and finite variance $\sigma^{\star 2}$,
\begin{equation}\label{ar1:eq:Hajek}
\forall \delta>0, \;  P \left( M_{n,1} \geq \delta^2 \right) \leq \frac{n\sigma^{\star 2}}{\delta^2} \; . 
\end{equation}
Letting $\delta^2 = \frac{n\Delta_n \beta_n}{8\left(m'+1\right)}$ in \eqref{ar1:eq:Hajek}, we get
\begin{equation*}
P\left( M_{n,1} \geq \frac{n\Delta_n \beta_n}{8\left(m'+1\right)} \right) 
\leq \frac{8\left(m'+1\right)\sigma^{\star 2}}{\Delta_n \beta_n}\;,
\end{equation*}
which goes to $0$ as $n$ tends to infinity because $\Delta_n \beta_n\underset{n\rightarrow\infty}{\longrightarrow} +\infty$. The proof of the convergence of $P\left( M_{n,2} \geq \frac{n\Delta_n \beta_n}{8\left(m'+1\right)} \right)$ follows the same lines.
\end{proof}

\subsection{Proof of Proposition \ref{ar1:Prop:SelBeta2}}\label{ar1:subsec:mbicbardet_bis}
\begin{lemma}\label{ar1:Lem:infSelBeta2}
Under the assumptions of Proposition \ref{ar1:Prop:SelBeta2}, $P\left(\widehat{m}=m\right)\underset{n\rightarrow\infty}{\longrightarrow} 0$ if $m<m^{\star}$.
\end{lemma}
\begin{lemma}\label{ar1:Lem:supSelBeta2}
Under the assumptions of Proposition \ref{ar1:Prop:SelBeta2}, $P\left(\widehat{m}=m\right)\underset{n\rightarrow\infty}{\longrightarrow} 0$ if $m>m^{\star}$.
\end{lemma}
\begin{proof}[Proof of Lemma \ref{ar1:Lem:infSelBeta2}]
Following the proof of Lemma \ref{ar1:Lem:infSelBeta} and replacing $\overline{w}$ by $\overline{v}$, we get, for any $\varepsilon >0$,
\begin{eqnarray}
P\left(\widehat{m}=m\right) & \leq & P\left(\exists \boldsymbol{t}'\in \mathcal{C}_{n,m^{\star},\nu} , J_n \left(\overline{v},\boldsymbol{t}'\right) \leq \varepsilon\right)\label{ar1:eq:ineq_inf_beta2}\\
 & \leq & P\left(\exists \boldsymbol{t}'\in \mathcal{C}_{n,m^{\star},\nu} , \frac{1}{2}K_n \left(\overline{w},\boldsymbol{t}'\right) + V_n\left(\overline{w},\boldsymbol{t}'\right) + W_n\left(\overline{w},\boldsymbol{t}'\right) \leq \frac{\varepsilon}{2}\right) \label{ar1:eq:ineq_inf_beta2_decompo}\\
 & + & P\left(\exists \boldsymbol{t}'\in \mathcal{C}_{n,m^{\star},\nu} , \frac{1}{2}K_n \left(\overline{w},\boldsymbol{t}'\right) + J_n \left(\overline{v},\boldsymbol{t}'\right) - J_n \left(\overline{w},\boldsymbol{t}'\right) \leq \frac{\varepsilon}{2}\right) \;, \nonumber
\end{eqnarray}
since
$$ J_n \left(\overline{v},\boldsymbol{t}'\right) = 
  \frac{1}{2}K_n \left(\overline{w},\boldsymbol{t}'\right) + V_n\left(\overline{w},\boldsymbol{t}'\right) + W_n\left(\overline{w},\boldsymbol{t}'\right)
  + 
  \frac{1}{2}K_n \left(\overline{w},\boldsymbol{t}'\right) + J_n \left(\overline{v},\boldsymbol{t}'\right) - J_n \left(\overline{w},\boldsymbol{t}'\right). $$
From \eqref{ar1:eq:demi} and \eqref{ar1:eq:ineq_inf_beta2_decompo}, it suffices to prove that
$$P\left(\exists \boldsymbol{t}'\in \mathcal{C}_{n,m^{\star},\nu} , \frac{1}{2}K_n \left(\overline{w},\boldsymbol{t}'\right) + J_n \left(\overline{v},\boldsymbol{t}'\right) - J_n \left(\overline{w},\boldsymbol{t}'\right) \leq \frac{\varepsilon}{2}\right)\underset{n\to\infty}{\longrightarrow}0  $$
to conclude the proof. It follows from \eqref{ar1:eq:controleunif} and \eqref{ar1:eq:HalfBound}, $\frac{1}{2}\underline{\lambda}^2 \nu$ being replaced by $\frac{1}{2}\left(\underline{\lambda}^2 \nu - \varepsilon\right)$, which is positive if $\varepsilon < \underline{\lambda}^2 \nu$.
\end{proof}
\begin{proof}[Proof of Lemma \ref{ar1:Lem:supSelBeta2}]
As in the proof of Lemma \ref{ar1:Lem:supSelBeta}, it suffices to show that 
$$P\left(\exists \boldsymbol{t}\in\mathcal{A}_{n,m}, J_n\left(\overline{v},\boldsymbol{t}\right) + \beta_n \leq 0\right)\underset{n\to\infty}{\longrightarrow} 0 \; .$$
Since $$J_n\left(\overline{v},\boldsymbol{t}\right)\geq J_n\left(\overline{w},\boldsymbol{t}\right) - \underset{t}{\sup}\left|J_n\left(\overline{v},\boldsymbol{t}\right) - J_n\left(\overline{w},\boldsymbol{t}\right)\right| \; , $$
the result follows from
\begin{eqnarray}
P\left(\exists \boldsymbol{t}\in\mathcal{A}_{n,m}, J_n\left(\overline{w},\boldsymbol{t}\right) + \frac{1}{2}\beta_n \leq 0\right) & \underset{n\to\infty}{\longrightarrow} & 0 \; , \label{ar1:eq:HalfBeta}\\
P\left(\underset{t}{\sup}\left|J_n\left(\overline{v},\boldsymbol{t}\right) - J_n\left(\overline{w},\boldsymbol{t}\right)\right| \geq \frac{1}{2}\beta_n\right)& \underset{n\to\infty}{\longrightarrow} & 0 \; . \label{ar1:eq:Diffvwbeta}
\end{eqnarray}
Equation~\eqref{ar1:eq:HalfBeta} follows from the Proof of Lemma~\ref{ar1:Lem:supSelBeta}, replacing $\beta_n$ by $\frac{1}{2}\beta_n$. Equation~\eqref{ar1:eq:Diffvwbeta} follows from~\eqref{ar1:eq:controleunif} and from $n^{1/2}\beta_n\underset{n\to\infty}{\longrightarrow} +\infty$.
\end{proof}

\subsection{Proof of Proposition \ref{ar1:Prop:mBICBardet}}\label{ar1:proof:Prop:mBICBardet}

We first give some lemmas which are useful for the proof of Proposition \ref{ar1:Prop:mBICBardet}.

\begin{lemma} \label{ar1:Lem:SSm} Under the assumptions of 
Proposition \ref{ar1:Prop:mBICBardet} with $SS_m$ given by \eqref{ar1:Eq:SSm}, we have, for any positive $m$,
$$
SS_m(z, \overline{\rho}_n) = SS_m(z, \rho^{\star}) + O_P(1),\textrm{ as } n\to\infty\;.
$$
\end{lemma}

\begin{lemma} \label{ar1:Lem:SSmstar} Under the assumptions of Proposition
\ref{ar1:Prop:mBICBardet} with $SS_m$ given by \eqref{ar1:Eq:SSm}, we have,
for any positive $m$,
$$
SS_m(z, \rho^{\star})^{-1} = O_P(n^{-1}),\textrm{ as } n\to\infty\;.
$$
\end{lemma}

%%%%%%%%%%%%%%%%%%%%%%%%%%%%%%%%%%%%%%%%%%%%%%%%%%%%%%%%%%%%%%%%%%%%%%%%%%%%%% 
\begin{proof}[Proof of Lemma \ref{ar1:Lem:SSm}]
 The proof of this Lemma follows exactly this of Lemma \ref{ar1:Lem:SSmY}. The difference is that, in \eqref{ar1:eq:bkw}, the term $\Delta^{\star}$ appearing in the decomposition \eqref{ar1:eq:dec:second:terme} vanishes.
\end{proof}

%%%%%%%%%%%%%%%%%%%%%%%%%%%%%%%%%%%%%%%%%%%%%%%%%%%%%%%%%%%%%%%%%%%%%%%%%%%%%% 
\begin{proof}[Proof of Lemma \ref{ar1:Lem:SSmstar}]
We first define 
$$
SS_m \left(z, \rho, \boldsymbol{t}\right) = \underset{\delta}{\argmin } SS_m \left(z, \rho, \delta, \boldsymbol{t} \right).
$$ 
We have, for any positive $M$, 
\begin{eqnarray*}
 P\left(\frac{n}{SS_m(z, \rho^{\star})} > M \right) 
 & \leq & P\left( \left\{\frac{SS_m(z, \rho^{\star})}{SS_m(z, \rho^{\star}, \boldsymbol{t^{\star}})} > 1 \right\} \bigcap \left\{\frac{n}{SS_m(z, \rho^{\star})} > M\right\} \right) \\
  & & + P\left( \left\{\frac{SS_m(z, \rho^{\star})}{SS_m(z, \rho^{\star}, \boldsymbol{t^{\star}})} < 1 \right\} \bigcap \left\{\frac{n}{SS_m(z, \rho^{\star})} > M\right\} \right) \\
  & \leq & P\left(\frac{n}{SS_m(z, \rho^{\star}, \boldsymbol{t^{\star}})} > M \right) + P\left(\frac{SS_m(z, \rho^{\star})}{SS_m(z, \rho^{\star}, \boldsymbol{t^{\star}})} < 1 \right).
\end{eqnarray*}
Under the assumptions of Proposition \ref{ar1:Prop:Segment}, a by product of the proof of Theorem 3 in \textcite{LM} is that
$$
P\left(\frac{SS_m(z, \rho^{\star})}{SS_m(z, \rho^{\star}, \boldsymbol{t^{\star}})} < 1 \right) = P\left(SS_m(z, \rho^{\star}) - SS_m(z, \rho^{\star}, \boldsymbol{t^{\star}}) < 0 \right) 
\leq \kappa n^{-\alpha},
$$
where $\kappa$ is a positive constant depending on $\boldsymbol{\delta^{\star}}$ and $\boldsymbol{t^{\star}}$, and $\alpha$ is a positive constant. 
Furthermore, as $\sigma^{\star -2}SS_m(z, \rho^{\star}, \boldsymbol{t^{\star}})$ has a $\chi^2_{n-m-1}$ distribution, 
$n^{-1}SS_m(z, \rho^{\star}, \boldsymbol{t^{\star}})=\sigma^{\star 2}+o_P(1)$ and thus {$n^{-1} SS_m(z, \rho^{\star}, \boldsymbol{t^{\star}})=O_P(1)$}, which concludes the proof.
\end{proof}

\begin{proof}[Proof of Proposition \ref{ar1:Prop:mBICBardet}]
We have to prove that, for a given positive $m$, $C_m(z, \rho^{\star}) - C_m(z, \overline{\rho}_n) = O_P(1)$. 
Observe that, since $\widehat{\tau}_k(z, \rho) = \widehat{t}_k(z, \rho) /n$, 
\begin{eqnarray} \label{ar1:Eq:DecompNkZ}
& & \sum_{k=0}^m \log n_k(\widehat{t}(z, \overline{\rho}_n)) - \sum_{k=0}^m \log
n_k(\widehat{t}(z, {\rho}^{\star})) \nonumber \\
& = & \sum_{k=0}^m \log (\widehat{\tau}_{k+1}(z, \overline{\rho}_n)-\widehat{\tau}_{k}(z, \overline{\rho}_n))- 
\sum_{k=0}^m \log (\widehat{\tau}_{k+1}(z, {\rho}^{\star})-\widehat{\tau}_{k}(z, {\rho}^{\star})).
\end{eqnarray}
By Proposition  \ref{ar1:Prop:Segment}, both quantities of the previous equation converge in probability
to $$\sum_{k=0}^m \log (\tau^{\star}_{k+1}-\tau^{\star}_{k}) \,$$
thus
\begin{equation} \label{ar1:Eq:CvgceNkZ}
\sum_{k=0}^m \log n_k(\widehat{t}(z, \overline{\rho}_n))- \sum_{k=0}^m \log
n_k(\widehat{t}(z, {\rho}^{\star}))=O_P(1). 
\end{equation}
Further note that
$$
\log {SS}_m(z, \overline{\rho}_n) - \log {SS}_m(z, {\rho}^{\star})
=\log\left(\frac{{SS}_m(z, \overline{\rho}_n)}{{SS}_m(z, {\rho}^{\star})}\right) 
= R\left(\frac{{SS}_m(z, \overline{\rho}_n)-{SS}_m(z, {\rho}^{\star})}{{SS}_m(z, {\rho}^{\star})}\right),
$$
where $R(x)=\log(1+x)$.
Lemma \ref{ar1:Lem:SSm} states that ${SS}_m(z, \overline{\rho}_n)-{SS}_m(z, {\rho}^{\star}) = O_P(1)$ and Lemma \ref{ar1:Lem:SSmstar} that $[{SS}_m(z, {\rho}^{\star})]^{-1} = O_P(n^{-1})$ so, by \textcite[Lemma 2.12]{van}, we get that
$$
\log {SS}_m(z, \overline{\rho}_n) - \log {SS}_m(z, {\rho}^{\star})
= O_P(n^{-1}).
$$
Hence
$$
\frac{n-m+1}{2} \log {SS}_m(z, \overline{\rho}_n) - \frac{n-m+1}{2} \log {SS}_m(z, {\rho}^{\star}) =
O_P(1),
$$
which with (\ref{ar1:Eq:CvgceNkZ}) concludes the proof of Proposition \ref{ar1:Prop:mBICBardet}.
\end{proof}

%%%%%%%%%%%%%%%%%%%%%%%%%%%%%%%%%%%%%%%%%%%%%%%%%%%%%%%%%%%%%%%%%%%%%%%%%%%%%%%%%%%%%%%%%%%%%
\subsection{Proof of Proposition \ref{ar1:Prop:mBIC}}\label{ar1:proof:Prop:mBIC}
We first give some lemmas which are useful for the proof of Proposition \ref{ar1:Prop:mBIC}.

\begin{lemma} \label{ar1:Lem:SSmY} Under the assumptions of 
Proposition \ref{ar1:Prop:mBICBardet} with $SS_m$ given by \eqref{ar1:Eq:SSm}, we have, for any positive $m$,
$$
SS_m(y, \overline{\rho}_n) = SS_m(y, \rho^{\star}) + O_P(1),\textrm{ as } n\to\infty\;.
$$
\end{lemma}

\begin{lemma} \label{ar1:Lem:SmYZ}
  If $(y_0, \dots y_n)$ is defined by \eqref{ar1:eq:modele_new} and $(z_0, \dots z_n)$ is defined as in Lemma \ref{ar1:Lem:YZ}, then 
  $$
  SS_m(y, {\rho}^{\star}) = SS_m(z, {\rho}^{\star}) + O_P(1),\textrm{ as } n\to\infty\;.
  $$
\end{lemma}

\begin{lemma} \label{ar1:Lem:OP1}
  Let  $(X_n)$ and $(Y_n)$ be two sequences of rv's such that $X_n - Y_n = O_P(1)$. If $Y_n ^{-1} = O_P(n^{-1})$ then $X_n ^{-1} = O_P(n^{-1})$.
\end{lemma}

%%%%%%%%%%%%%%%%%%%%%%%%%%%%%%%%%%%%%%%%%%%%%%%%%%%%%%%%%%%%%%%%%%%%%%%%%%%%%% 
\begin{proof}[Proof of Lemma \ref{ar1:Lem:SSmY}]
Using the matrix notations from the proof of Lemma \ref{ar1:Lem:Delta_order}, we have
$$
SS_m(y, \rho^{\star}) = \min_{T, \delta} \Vert y - \rho^{\star} By - T \delta \Vert^2, 
\qquad
SS_m(y, \overline{\rho}_n) = \min_{T, \delta} \Vert y - \overline{\rho}_n  By - T \delta \Vert^2,
$$
where all minimizations are achieved over all segmentations with $m$ change points belonging to $\mathcal{A}_{n,m}$. 
Let us define $(\widehat{T}^{\star}, \widehat{\delta}^{\star})$
and $(\overline{T}, \overline{\delta})$ by 
\begin{equation*}
(\widehat{T}^{\star}, \widehat{\delta}^{\star}) = \argmin_{T, \delta} \Vert y - \rho^{\star}By - T\delta \Vert, 
\qquad
(\overline{T}, \overline{\delta}) = \argmin_{T, \delta} \Vert y - \overline{\rho}_n By - T\delta \Vert.
\end{equation*}
Note that $\widehat{T}^{\star}$ and $\overline{T}$ refer to $\widehat{t}(y, \rho^{\star})$ and $\widehat{t}(y, \overline{\rho}_n)$, respectively. We have 
\begin{eqnarray} \label{ar1:Eq:UpperBoundSSdiff}
 \left| SS_m(y, \overline{\rho}_n) - SS_m(y, \rho^{\star}) \right| 
 & = &  \left| \min_{T, \delta} \Vert y - \overline{\rho}_n By - T\delta \Vert^2 - \min_{T, \delta} \Vert y - \rho^{\star} By - T\delta \Vert^2 \right| \nonumber \\
 & \leq & 
 \max \left( \left| \Vert y - \overline{\rho}_n By - \widehat{T}^{\star}\widehat{\delta}^{\star} \Vert^2 - \Vert y - \rho^{\star}By - \widehat{T}^{\star}\widehat{\delta}^{\star} \Vert^2 \right|, \right. \nonumber\\
  & & \qquad \left. \left| \Vert y - \overline{\rho}_n By - \overline{T}\,\overline{\delta} \Vert^2 - \Vert y - \rho^{\star}By - \overline{T}\,\overline{\delta} \Vert^2 \right| \right).
\end{eqnarray}
We now have to prove that this upper bound is $O_P(1)$. We first prove it for the second term of in the right-hand side of \eqref{ar1:Eq:UpperBoundSSdiff}. To do so, observe that
$\Vert y - \overline{\rho}_n By - \overline{T}\,\overline{\delta} \Vert^2
=\Vert y - \rho^{\star}By - \overline{T}\,\overline{\delta}+(\rho^{\star}-\overline{\rho}_n) By\Vert^2$. Thus,
$$
\Vert y - \overline{\rho}_n By - \overline{T}\overline{\delta} \Vert^2 - \Vert y - \rho^{\star}By - \overline{T}\overline{\delta} \Vert^2 
=(\overline{\rho}_n  - \rho^{\star})^2 \Vert By\Vert^2 +2(\rho^{\star}-\overline{\rho}_n)\langle By,y - \rho^{\star}By - \overline{T}\,\overline{\delta} \rangle.
$$
Since, by (\ref{ar1:eq:modele_matriciel}) and Lemma \ref{ar1:Lem:YZ}, $y - \rho^{\star}By - \overline{T}\,\overline{\delta}
=\epsilon - \Delta^{\star} + (T^{\star}\delta^{\star}-\overline{T}\,\overline{\delta})=\epsilon- \Delta^{\star}
+T^{\star}(\delta^{\star}-\overline{\delta})+(T^{\star}-\overline{T})\overline{\delta}$, where $\Delta^{\star}$ is the $n$-dimensional vector with entries $\Delta^{\star}_i$, we get
\begin{multline}\label{ar1:eq:dec:second:terme}
\Vert y - \overline{\rho}_n By - \overline{T}\,\overline{\delta} \Vert^2 - \Vert y - \rho^{\star}By - \overline{T}\,\overline{\delta} \Vert^2\\
=(\overline{\rho}_n  - \rho^{\star})^2 \Vert By\Vert^2 
+ 2 (\rho^{\star}- \overline{\rho}_n ) \left(\langle By,\epsilon  \rangle + \langle By,T^{\star} (\delta^{\star} - \overline{\delta} )  \rangle 
+ \langle By,(T^{\star}-\overline{T}) \overline{\delta}  \rangle - \langle By, \Delta^{\star}\rangle \right).
\end{multline}
Let us now prove that each term in the right-hand side of (\ref{ar1:eq:dec:second:terme}) is $O_P(1)$.
\begin{enumerate}[($a$)]
\item Let us study the first term of (\ref{ar1:eq:dec:second:terme}).
Using Lemma \ref{ar1:lem:rateXY} and (\ref{ar1:eq:hypRhoRate}) we get that 
  \begin{equation}\label{ar1:Eq:rhoXnorm}
  (\overline{\rho}_n -\rho^{\star})^2 \Vert By\Vert^2 = O_P(1).
  \end{equation}
\item Let us now study the second term of (\ref{ar1:eq:dec:second:terme}). Observe that 
$
\left\langle By,\epsilon\right\rangle = \sum_{i=1}^n y_{i-1}\epsilon_i=\sum_{i=1}^n (y_{i-1}-\PE(y_{i-1}))\epsilon_i+\sum_{i=1}^n \PE(y_{i-1})\epsilon_i.
$
By using the Central limit theorem for  iid rv's and since there is a finite number of change-points, the second term
is $O_P(\sqrt{n})$. As for the first term, since $(y_{i-1}-\PE(y_{i-1}))$ is a causal AR(1) process, then by using the beginning of the proof of Proposition 8.10.1 of \textcite{brockwell}, we get
that $\sum_{i=1}^n (y_{i-1}-\PE(y_{i-1}))\epsilon_i=O_P (\sqrt{n})$. Thus,
  \begin{equation} \label{ar1:Eq:CrossProd1}  
  \left\langle By,\epsilon\right\rangle %= \sum_{i=1}^n y_{i-1}\epsilon_i 
= O_P (\sqrt{n}).
 \end{equation}
  Furthermore, we have $\Vert T^{\star} ( \delta^{\star} - \overline{\delta} ) \Vert^2 = \sum_{k=0}^{m}\left(t_{k+1}^{\star}-t_k^{\star}\right) (\delta^{\star}_k -\overline{\delta}_k)^2$ 
 where each term of the sum is $O_P(1)$, thanks to Proposition \ref{ar1:Prop:Segment2}, and so is the sum. 
Now using Lemma \ref{ar1:lem:rateXY} and the Cauchy-Schwarz inequality, we get 
\begin{equation} \label{ar1:Eq:CrossProd2}  
  \langle By, T^{\star} ( \delta^{\star} - \overline{\delta} )  \rangle = O_P(\sqrt{n}).
  \end{equation}
  The convergence rate of $\widehat{t}(y,\overline{\rho}_n)$ given in Proposition \ref{ar1:Prop:Segment2} ensures that, for any $\varepsilon>0$ there exists a positive $M$ 
such that each column of $(T^{\star} - \overline{T})$ has at most $M$ non-zero coefficients with probability greater than $1-\varepsilon$. 
By using Proposition \ref{ar1:Prop:Segment2}, we obtain that with probability greater than $1-\varepsilon$
  \begin{equation}\label{ar1:eq:T*-Tbar}
  \Vert(T^{\star} - \overline{T}) \overline{\delta} \Vert^2 \leq M \sum_k \overline{\delta}_k^2 =2 M \sum_k (\overline{\delta}_k-\delta^{\star}_k)^2
+2M \sum_k {\delta^{\star}_k}^2\leq MM',
\end{equation}
where $M'$ is a positive constant. 
By the Cauchy-Schwarz inequality, (\ref{ar1:eq:T*-Tbar}) and Lemma \ref{ar1:lem:rateXY}, we get 
  \begin{equation} \label{ar1:Eq:CrossProd3}  
  \langle By, (T^{\star} - \overline{T}) \overline{\delta}  \rangle = O_P (\sqrt{n}).
  \end{equation}
  As $\Delta^{\star}$ has only $m$ non-zero entries, $\langle By, \Delta^{\star}\rangle$ is the sum of $m$ Gaussian rv's and is therefore $O_P(1)$.
  
  Thus, combining \eqref{ar1:Eq:CrossProd1}, \eqref{ar1:Eq:CrossProd2} and \eqref{ar1:Eq:CrossProd3} with (\ref{ar1:eq:hypRhoRate}), we get
  $$
  (\rho^{\star}- \overline{\rho}_n ) \left(\langle By,\epsilon  \rangle + \langle By,T^{\star} (\delta^{\star} - \overline{\delta} )  \rangle + \langle By,(T^{\star} - \overline{T}) \overline{\delta}  \rangle -  \langle By, \Delta^{\star}\rangle \right) = O_P(1).
  $$
\end{enumerate}

To complete the proof, we need to consider the first term of \eqref{ar1:Eq:UpperBoundSSdiff}.
As $\rho^{\star}$ satisfies the same assumptions as $\overline{\rho}_n$, using the same line of reasoning as for the second term holds so we get
$$
\Vert y - \overline{\rho}_n By - \widehat{T}^{\star}\widehat{\delta}^{\star} \Vert^2 - \Vert y - \rho^{\star}By - \widehat{T}^{\star}\widehat{\delta}^{\star} \Vert^2 = O_P(1).
$$

\end{proof}

%%%%%%%%%%%%%%%%%%%%%%%%%%%%%%%%%%%%%%%%%%%%%%%%%%%%%%%%%%%%%%%%%%%%%%%%%%%%%% 
\begin{proof}[Proof of Lemma \ref{ar1:Lem:SmYZ}] 
The proof follows the same line of reasoning as the proof of Lemma \ref{ar1:Lem:SSmY}.

Let us define $(\widehat{T}^y, \widehat{\delta}^y)$
and $(\widehat{T}^z, \widehat{\delta}^z)$ by 
\begin{equation*}
(\widehat{T}^y, \widehat{\delta}^y)
= \argmin_{T, \delta} 
\Vert y - \rho^{\star} By - T \delta \Vert^2,
\qquad
(\widehat{T}^z, \widehat{\delta}^z)
= \argmin_{T, \delta} 
\Vert z - \rho^{\star} Bz - T \delta \Vert^2.
\end{equation*}
We have 
\begin{multline*} 
\left|SS_m(y, \rho^{\star}) - SS_m(z, \rho^{\star}) \right\| 
 \leq 
 \max \left( \left| \Vert y - \rho^{\star} By - \widehat{T}^y \widehat{\delta}^y \Vert^2 - \Vert z - \rho^{\star}Bz - \widehat{T}^y \widehat{\delta}^y \Vert^2 \right|, \right. \\
 \left. \left| \Vert y - \rho^{\star} By - \widehat{T}^z \widehat{\delta}^z \Vert^2 - \Vert z - \rho^{\star}Bz - \widehat{T}^z \widehat{\delta}^z \Vert^2 \right| \right).
\end{multline*}
According to Lemma \ref{ar1:Lem:YZ}, we have $y - \rho^{\star} By = z - \rho^{\star} Bz - \Delta^{\star}$ where $\Delta^{\star}=(\Delta_i^{\star})$. As for the first term
\begin{multline*}
\Vert y - \rho^{\star} By - \widehat{T}^y \widehat{\delta}^y \Vert^2 - \Vert z - \rho^{\star}Bz - \widehat{T}^y \widehat{\delta}^y \Vert^2 \\
= \Vert \Delta^{\star} \Vert^2 
- 2 \left(\langle \Delta^{\star},\epsilon \rangle + \langle \Delta^{\star}, T^{\star} (\delta^{\star} - \widehat{\delta}^y )  \rangle 
+ \langle \Delta^{\star},(T^{\star}-\widehat{T}^y) \widehat{\delta}^y \rangle \right),
\end{multline*}
the first term of which is a constant and all other terms being $O_P(1)$, which can be proved following the same line as the proof of Lemma \ref{ar1:Lem:SSmY}. The control of $\Vert y - \rho^{\star} By - \widehat{T}^z \widehat{\delta}^z \Vert^2 - \Vert z - \rho^{\star}Bz - \widehat{T}^z \widehat{\delta}^z \Vert^2$ follows the same lines.
  \end{proof}

%%%%%%%%%%%%%%%%%%%%%%%%%%%%%%%%%%%%%%%%%%%%%%%%%%%%%%%%%%%%%%%%%%%%%%%%%%%%%% 
\begin{proof}[Proof of Lemma \ref{ar1:Lem:OP1}]
Observe that 
$$X_n^{-1}=\left(Y_n+(X_n-Y_n)\right)^{-1}=Y_n^{-1}\left(1+Y_n^{-1}(X_n-Y_n)\right)^{-1}\; .$$
Since, by assumption, $Y_n^{-1}(X_n-Y_n)=O_P(n^{-1})$, the terms inside
the parentheses converges in probability to one. Thus, $\left(1+Y_n^{-1}(X_n-Y_n)\right)^{-1}$ is in particular $O_P(1)$ which concludes the proof.
\end{proof}

\begin{proof}[Proof of Proposition \ref{ar1:Prop:mBIC}]
   As for the proof of Proposition \ref{ar1:Prop:mBICBardet}, denoting $\widehat{\tau}_k(y, \rho) = \widehat{t}_k(y, \rho) /n$, the decomposition \eqref{ar1:Eq:DecompNkZ} still holds, replacing $z$ with $y$. Then, by Proposition~\ref{ar1:Prop:Segment2}, we have
   $$
   \sum_{k=0}^m \log n_k(\widehat{t}(y, \overline{\rho}_n))- \sum_{k=0}^m \log
   n_k(\widehat{t}(y, {\rho}^{\star}))=O_P(1). 
   $$
   For a process $y$ under Model~\eqref{ar1:eq:modele_new}, we construct a process $z$ under Model~\eqref{ar1:eq:bkw} using Lemma~\ref{ar1:Lem:YZ}. The proof relies on the fact that $y$ inherits some properties of $z$. Again, we note that
   $$
   \log {SS}_m(y, \overline{\rho}_n) - \log {SS}_m(y, {\rho}^{\star})
    = R\left(\frac{{SS}_m(y, \overline{\rho}_n)-{SS}_m(y, {\rho}^{\star})}{{SS}_m(y, {\rho}^{\star})}\right).
   $$
  Lemma \ref{ar1:Lem:SSmY} states that ${SS}_m(y, \overline{\rho}_n)-{SS}_m(y, {\rho}^{\star}) = O_P(1)$. 
  To conclude the proof we need to further show that $[{SS}_m(y, {\rho}^{\star})]^{-1} = O_P(n^{-1})$. We first show that $[{SS}_m(y, {\rho}^{\star}) - {SS}_m(z, {\rho}^{\star})] = O_P(1)$ in Lemma~\ref{ar1:Lem:SmYZ} and, because $[{SS}_m(z, {\rho}^{\star})]^{-1} = O_P(n^{-1})$, we conclude using Lemma~\ref{ar1:Lem:OP1}.
\end{proof}

%%% Local Variables:
%%% mode: latex
%%% eval: (TeX-PDF-mode 1)
%%% TeX-master: "article.tex"
%%% ispell-local-dictionary: "en_US"
%%% eval: (flyspell-mode 1)
%%% End: 

%%% Local Variables:
%%% mode: latex
%%% eval: (TeX-PDF-mode 1)
%%% TeX-master: "article.tex"
%%% ispell-local-dictionary: "en_US"
%%% eval: (flyspell-mode 1)
%%% End: 
