# Supplementary material for: A robust approach for estimating change-points in the mean of an AR(p) process
Source: arXiv:1509.00899 source file (2015-09-02)
Supplement: Supplementary file 2 [file AppSec4.tex]

\subsection{Proof of Proposition \ref{ar1:Prop:SelBeta}}\label{ar1:subsec:bicbardet}
We shall used in this section the notations introduced in Sections \ref{ar1:subsec:prop:Segment} and \ref{ar1:subsec:beta}.
 The result derives directly from Lemmas \ref{ar1:Lem:infSelBeta} and \ref{ar1:Lem:supSelBeta}.
 
\begin{lemma}\label{ar1:Lem:infSelBeta}
Under the assumptions of Proposition \ref{ar1:Prop:SelBeta}, $P\left(\widehat{m}=m\right)\underset{n\rightarrow\infty}{\longrightarrow} 0$ if $m<m^{\star}$.
\end{lemma}
\begin{lemma}\label{ar1:Lem:supSelBeta}
Under the assumptions of Proposition \ref{ar1:Prop:SelBeta}, $P\left(\widehat{m}=m\right)\underset{n\rightarrow\infty}{\longrightarrow} 0$ if $m>m^{\star}$.
\end{lemma}

\begin{proof}[Proof of Lemma \ref{ar1:Lem:infSelBeta}]
If $\widehat{m}=m<m^{\star}$, then
\begin{equation*}
\frac1n SS_m(z, \overline{\rho}_n) + \beta_n m \leq \frac1n SS_{m^{\star}}(z, \overline{\rho}_n) + \beta_n m^{\star} \; ,
\end{equation*}
where $SS_m$ is defined in \eqref{ar1:Eq:SSm}. In particular, there exists $\boldsymbol{t}\in \mathcal{A}_{n,m}$ such that
\begin{equation*}
\frac1n \underset{\boldsymbol{\delta}}{\min} SS_m(z, \overline{\rho}_n, \boldsymbol{\delta}, \boldsymbol{t}) + \beta_n m \leq \frac1n \underset{\boldsymbol{\delta}}{\min} SS_m(z, \overline{\rho}_n, \boldsymbol{\delta}, \boldsymbol{t}_n^{\star}) + \beta_n m^{\star} \; .
\end{equation*}
From \eqref{ar1:eq:Jnm}, we get
\begin{equation*}
J_n \left(\overline{w},\boldsymbol{t}\right) \leq \beta_n\left(m^{\star} - m\right) \; .
\end{equation*}
Since $\left(\beta_n\right)$ converges to zero, for any $\varepsilon>0$, $\beta_n\left(m^{\star} - m\right) \leq \varepsilon$ for a large
enough $n$, and so
\begin{equation*}
J_n \left(\overline{w},\boldsymbol{t}\right) \leq \varepsilon \; .
\end{equation*}
One can check that there exist $0<\nu<\Delta_{\boldsymbol{\tau}^{\star}}$ such that, for a large enough $n$, there exists $\boldsymbol{t}'\in \mathcal{C}_{n,m^{\star},\nu}$ such that $E_{\boldsymbol{t}} \subset E_{\boldsymbol{t}'}$ (that is the change-points of $\boldsymbol{t}$ are change-points of $\boldsymbol{t}'$) for all $\boldsymbol{t}\in \mathcal{A}_{n,m}$, where $\mathcal{C}_{n,m^{\star},\nu}$ is defined in \eqref{ar1:eq:Cn_alpha}. From \eqref{ar1:eq:Jnm} and $E_{\boldsymbol{t}} \subset E_{\boldsymbol{t}'}$, we get $J_n \left(\overline{w},\boldsymbol{t}'\right) \leq J_n \left(\overline{w},\boldsymbol{t}\right)$. Then, the following inequality holds for all $\varepsilon>0$ and any large enough $n$:
\begin{equation}\label{ar1:eq:ineq_inf_beta}
P\left(\widehat{m}=m\right) \leq P\left(\exists \boldsymbol{t}'\in \mathcal{C}_{n,m^{\star},\nu} , J_n \left(\overline{w},\boldsymbol{t}'\right) \leq \varepsilon\right) \; .
\end{equation}
We then follow the steps of \eqref{ar1:eq:ineq_alpha}, $-\nu\underline{\lambda}^2$ being replaced by $\varepsilon-\nu\underline{\lambda}^2$. The convergence of $P\left(\exists \boldsymbol{t}'\in \mathcal{C}_{n,m^{\star},\nu} , J_n \left(\overline{w},\boldsymbol{t}'\right) \leq \varepsilon\right)$ to zero holds with $\varepsilon < \nu\underline{\lambda}^2$. We can conclude with \eqref{ar1:eq:ineq_inf_beta}.
\end{proof}
\begin{proof}[Proof of Lemma \ref{ar1:Lem:supSelBeta}]
Following the proof of Lemma \ref{ar1:Lem:infSelBeta}, if $\widehat{m}=m>m^{\star}$, there exists $\boldsymbol{t}\in\mathcal{A}_{n,m}$ such that $J_n \left(\overline{w},\boldsymbol{t}\right) \leq \beta_n\left(m^{\star} - m\right)$ and then $ J_n \left(\overline{w},\boldsymbol{t}\right) + \beta_n \leq 0 $ since $m>m^{\star}$. Then
\begin{equation}\label{ar1:eq:ineq_sup_beta}
P\left(\widehat{m}=m\right) \leq P\left(\exists \boldsymbol{t}\in \mathcal{A}_{n,m} , J_n \left(\overline{w},\boldsymbol{t}\right) + \beta_n \leq 0\right) \; .
\end{equation}
Adding the change-points of $\boldsymbol{t}_n^{\star}$ to those of such a $\boldsymbol{t}$, one can get $t'\in\mathcal{A}_{n,m'}$ with $m^{\star}<m\leq m' \leq m+m^{\star}$ such that $E_{\boldsymbol{t}}\cup E_{\boldsymbol{t}_n^{\star}}\subset E_{\boldsymbol{t}'}$, provided that $\left(m+m^{\star}\right)\left\lceil\Delta_n\right\rceil\leq n$, where $\lceil\cdot \rceil$ is the ceiling function, this condition being fulfilled for any sufficiently large $n$ under the assumptions of Proposition \ref{ar1:Prop:SelBeta} since $n^{-1}\Delta_n$ converges to zero. Since $E_{\boldsymbol{t}}\subset E_{\boldsymbol{t}'}$, we derive $J_n \left(\overline{w},\boldsymbol{t}'\right)+ \beta_n \leq J_n \left(\overline{w},\boldsymbol{t}\right) + \beta_n$ from \eqref{ar1:eq:Jnm}. Then, from \eqref{ar1:eq:ineq_sup_beta}, we get
\begin{equation}\label{ar1:eq:sublemma_sup_beta}
\forall m' > m^{\star} , P\left(\exists \boldsymbol{t}'\in \mathcal{A}_{n,m'} , E_{\boldsymbol{t}_n^{\star}}\subset E_{\boldsymbol{t}'},  J_n \left(\overline{w},\boldsymbol{t}'\right)+ \beta_n \leq 0\right) \underset{n\rightarrow\infty}{\longrightarrow} 0
\end{equation}
is a sufficient condition to prove the lemma. Let us prove \eqref{ar1:eq:sublemma_sup_beta}. Let $m'>m^{\star}$ and such a $\boldsymbol{t}'$. We compare $J_n \left(\overline{w},\boldsymbol{t}'\right)$ to $J_n \left(w^{\star},\boldsymbol{t}'\right)$. Since $\mathbb{E}w^{\star}\in E_{\boldsymbol{t}_n^{\star}}\subset E_{\boldsymbol{t}'}$, $K_n \left(w^{\star} , \boldsymbol{t}'\right) = 0$ by \eqref{ar1:eq:Kn}. By~\eqref{ar1:eq:Wn} and $\mathbb{E}w^{\star}\in E_{\boldsymbol{t}_n^{\star}}\subset E_{\boldsymbol{t}'}$,
\begin{eqnarray*}
W_n\left(w^{\star},\boldsymbol{t}'\right) & = & \frac{2}{n}\left( \left\langle \pi_{E_{\boldsymbol{t}_n^{\star}}} \left( w^{\star}-\mathbb{E}w^{\star}\right), \pi_{E_{\boldsymbol{t}_n^{\star}}} \left( \mathbb{E}w^{\star} \right)\right\rangle - \left\langle \pi_{E_{\boldsymbol{t}'}} \left( w^{\star}-\mathbb{E}w^{\star}\right), \pi_{E_{\boldsymbol{t}'}} \left( \mathbb{E}w^{\star} \right)\right\rangle  \right)\\
 & = & \frac{2}{n}\left\langle \pi_{E_{\boldsymbol{t}_n^{\star}}} \left( w^{\star}-\mathbb{E}w^{\star}\right) - \pi_{E_{\boldsymbol{t}'}} \left( w^{\star}-\mathbb{E}w^{\star}\right), \pi_{E_{\boldsymbol{t}_n^{\star}}} \left( \mathbb{E}w^{\star} \right)\right\rangle \\
  & = & - \frac{2}{n}\left\langle \pi_{E_{\boldsymbol{t}_n^{\star}}^\bot} \pi_{E_{\boldsymbol{t}'}} \left( w^{\star}-\mathbb{E}w^{\star}\right), \pi_{E_{\boldsymbol{t}_n^{\star}}} \left( \mathbb{E}w^{\star} \right)\right\rangle \\
   & = & 0 \; ,
\end{eqnarray*}
where $E^\bot$ is the (Euclidian) orthogonal complement of the vector subspace $E$. Then $J_n \left(w^{\star},\boldsymbol{t}'\right) = V_n \left(w^{\star},\boldsymbol{t}'\right)$ and
\begin{equation}\label{ar1:eq:decomp_sup_beta}
J_n \left(\overline{w},\boldsymbol{t}'\right) = V_n \left(w^{\star},\boldsymbol{t}'\right) + \left(J_n \left(\overline{w},\boldsymbol{t}'\right) - J_n \left(w^{\star},\boldsymbol{t}'\right)\right) \; .
\end{equation}
Using \eqref{ar1:eq:LMboundV}, $V_n\left(w^{\star},\boldsymbol{t}\right)  \geq  -\frac{2\left(m'+1\right)}{n\Delta_n}M_n$, where
\begin{eqnarray*}
M_n & = & M_{n,1} + M_{n,2}\;,\\
 M_{n,1} & = & \max_{1\leq s\leq n} \left(\sum_{i=1}^s \epsilon_i\right)^2\;, \\
 M_{n,2} & = &  \max_{1\leq s\leq n} \left(\sum_{i=n-s}^{n} \epsilon_i\right)^2\;.
\end{eqnarray*}
 We define $D_n = \underset{\boldsymbol{t}' \in\mathcal{A}_{n,m'}}{\sup} \left| J_n \left(\overline{w},\boldsymbol{t}'\right) - J_n \left(w^{\star},\boldsymbol{t}'\right) \right|$. Then, using \eqref{ar1:eq:decomp_sup_beta},
\begin{equation*}
J_n \left(\overline{w},\boldsymbol{t}'\right) \geq -\frac{2\left(m+1\right)}{n\Delta_n}M_n - D_n \; ,
\end{equation*}
which implies
\begin{eqnarray*}
P\left(\exists \boldsymbol{t}'\in \mathcal{A}_{n,m'} , E_{\boldsymbol{t}_n^{\star}}\subset E_{\boldsymbol{t}'},  J_n \left(\overline{w},\boldsymbol{t}'\right)+ \beta_n \leq 0\right) & \leq & P\left( -\frac{2\left(m'+1\right)}{n\Delta_n}M_n - D_n + \beta_n \leq 0\right)\\
 & \leq & P\left( \frac{2\left(m'+1\right)}{n\Delta_n}M_n \geq \frac{\beta_n}{2} \right) + P\left(  D_n \geq \frac{\beta_n}{2} \right) \; .
\end{eqnarray*}
By Lemma \ref{ar1:lem:BoundedUnifBound}, $D_n = O_P \left(n^{-1/2}\right)$ and then $P\left(  D_n \geq \frac{\beta_n}{2} \right)$ tends to zero as $n$ tends to infinity since $n^{1/2}\beta_n\underset{n\rightarrow\infty}{\longrightarrow} + \infty $. Let us now prove that $P\left( \frac{2\left(m+1\right)}{n\Delta_n}M_n \geq \frac{\beta_n}{2} \right)$ tends to zero as $n$ tends to infinty, which concludes the proof. Note that
\begin{equation*}
P\left( \frac{2\left(m'+1\right)}{n\Delta_n}M_n \geq \frac{\beta_n}{2} \right) \leq P\left( M_{n,1} \geq \frac{n\Delta_n \beta_n}{8\left(m'+1\right)} \right) + P\left( M_{n,2} \geq \frac{n\Delta_n \beta_n}{8\left(m'+1\right)} \right) \; .
\end{equation*}
We prove the convergence for each term in the right-hand side of the above equation. We shall prove it for the first term in the right-hand side since the arguments for the other term are the same.  From  Kolmogorov's maximal inequality \parencite[see for example][Theorem 2.5.2.]{durrett2010probability}\footnote{See Theorem~\ref{th:kolmogorov} of this document.}, since $\left(\epsilon_i\right)_{i\geq 0}$ is a sequence of independent rv's with zero-mean and finite variance $\sigma^{\star 2}$,
\begin{equation}\label{ar1:eq:Hajek}
\forall \delta>0, \;  P \left( M_{n,1} \geq \delta^2 \right) \leq \frac{n\sigma^{\star 2}}{\delta^2} \; . 
\end{equation}
Letting $\delta^2 = \frac{n\Delta_n \beta_n}{8\left(m'+1\right)}$ in \eqref{ar1:eq:Hajek}, we get
\begin{equation*}
P\left( M_{n,1} \geq \frac{n\Delta_n \beta_n}{8\left(m'+1\right)} \right) 
\leq \frac{8\left(m'+1\right)\sigma^{\star 2}}{\Delta_n \beta_n}\;,
\end{equation*}
which goes to $0$ as $n$ tends to infinity because $\Delta_n \beta_n\underset{n\rightarrow\infty}{\longrightarrow} +\infty$. The proof of the convergence of $P\left( M_{n,2} \geq \frac{n\Delta_n \beta_n}{8\left(m'+1\right)} \right)$ follows the same lines.
\end{proof}

\subsection{Proof of Proposition \ref{ar1:Prop:SelBeta2}}\label{ar1:subsec:mbicbardet_bis}
\begin{lemma}\label{ar1:Lem:infSelBeta2}
Under the assumptions of Proposition \ref{ar1:Prop:SelBeta2}, $P\left(\widehat{m}=m\right)\underset{n\rightarrow\infty}{\longrightarrow} 0$ if $m<m^{\star}$.
\end{lemma}
\begin{lemma}\label{ar1:Lem:supSelBeta2}
Under the assumptions of Proposition \ref{ar1:Prop:SelBeta2}, $P\left(\widehat{m}=m\right)\underset{n\rightarrow\infty}{\longrightarrow} 0$ if $m>m^{\star}$.
\end{lemma}
\begin{proof}[Proof of Lemma \ref{ar1:Lem:infSelBeta2}]
Following the proof of Lemma \ref{ar1:Lem:infSelBeta} and replacing $\overline{w}$ by $\overline{v}$, we get, for any $\varepsilon >0$,
\begin{eqnarray}
P\left(\widehat{m}=m\right) & \leq & P\left(\exists \boldsymbol{t}'\in \mathcal{C}_{n,m^{\star},\nu} , J_n \left(\overline{v},\boldsymbol{t}'\right) \leq \varepsilon\right)\label{ar1:eq:ineq_inf_beta2}\\
 & \leq & P\left(\exists \boldsymbol{t}'\in \mathcal{C}_{n,m^{\star},\nu} , \frac{1}{2}K_n \left(\overline{w},\boldsymbol{t}'\right) + V_n\left(\overline{w},\boldsymbol{t}'\right) + W_n\left(\overline{w},\boldsymbol{t}'\right) \leq \frac{\varepsilon}{2}\right) \label{ar1:eq:ineq_inf_beta2_decompo}\\
 & + & P\left(\exists \boldsymbol{t}'\in \mathcal{C}_{n,m^{\star},\nu} , \frac{1}{2}K_n \left(\overline{w},\boldsymbol{t}'\right) + J_n \left(\overline{v},\boldsymbol{t}'\right) - J_n \left(\overline{w},\boldsymbol{t}'\right) \leq \frac{\varepsilon}{2}\right) \;, \nonumber
\end{eqnarray}
since
$$ J_n \left(\overline{v},\boldsymbol{t}'\right) = 
  \frac{1}{2}K_n \left(\overline{w},\boldsymbol{t}'\right) + V_n\left(\overline{w},\boldsymbol{t}'\right) + W_n\left(\overline{w},\boldsymbol{t}'\right)
  + 
  \frac{1}{2}K_n \left(\overline{w},\boldsymbol{t}'\right) + J_n \left(\overline{v},\boldsymbol{t}'\right) - J_n \left(\overline{w},\boldsymbol{t}'\right). $$
From \eqref{ar1:eq:demi} and \eqref{ar1:eq:ineq_inf_beta2_decompo}, it suffices to prove that
$$P\left(\exists \boldsymbol{t}'\in \mathcal{C}_{n,m^{\star},\nu} , \frac{1}{2}K_n \left(\overline{w},\boldsymbol{t}'\right) + J_n \left(\overline{v},\boldsymbol{t}'\right) - J_n \left(\overline{w},\boldsymbol{t}'\right) \leq \frac{\varepsilon}{2}\right)\underset{n\to\infty}{\longrightarrow}0  $$
to conclude the proof. It follows from \eqref{ar1:eq:controleunif} and \eqref{ar1:eq:HalfBound}, $\frac{1}{2}\underline{\lambda}^2 \nu$ being replaced by $\frac{1}{2}\left(\underline{\lambda}^2 \nu - \varepsilon\right)$, which is positive if $\varepsilon < \underline{\lambda}^2 \nu$.
\end{proof}
\begin{proof}[Proof of Lemma \ref{ar1:Lem:supSelBeta2}]
As in the proof of Lemma \ref{ar1:Lem:supSelBeta}, it suffices to show that 
$$P\left(\exists \boldsymbol{t}\in\mathcal{A}_{n,m}, J_n\left(\overline{v},\boldsymbol{t}\right) + \beta_n \leq 0\right)\underset{n\to\infty}{\longrightarrow} 0 \; .$$
Since $$J_n\left(\overline{v},\boldsymbol{t}\right)\geq J_n\left(\overline{w},\boldsymbol{t}\right) - \underset{t}{\sup}\left|J_n\left(\overline{v},\boldsymbol{t}\right) - J_n\left(\overline{w},\boldsymbol{t}\right)\right| \; , $$
the result follows from
\begin{eqnarray}
P\left(\exists \boldsymbol{t}\in\mathcal{A}_{n,m}, J_n\left(\overline{w},\boldsymbol{t}\right) + \frac{1}{2}\beta_n \leq 0\right) & \underset{n\to\infty}{\longrightarrow} & 0 \; , \label{ar1:eq:HalfBeta}\\
P\left(\underset{t}{\sup}\left|J_n\left(\overline{v},\boldsymbol{t}\right) - J_n\left(\overline{w},\boldsymbol{t}\right)\right| \geq \frac{1}{2}\beta_n\right)& \underset{n\to\infty}{\longrightarrow} & 0 \; . \label{ar1:eq:Diffvwbeta}
\end{eqnarray}
Equation~\eqref{ar1:eq:HalfBeta} follows from the Proof of Lemma~\ref{ar1:Lem:supSelBeta}, replacing $\beta_n$ by $\frac{1}{2}\beta_n$. Equation~\eqref{ar1:eq:Diffvwbeta} follows from~\eqref{ar1:eq:controleunif} and from $n^{1/2}\beta_n\underset{n\to\infty}{\longrightarrow} +\infty$.
\end{proof}

\subsection{Proof of Proposition \ref{ar1:Prop:mBICBardet}}\label{ar1:proof:Prop:mBICBardet}

We first give some lemmas which are useful for the proof of Proposition \ref{ar1:Prop:mBICBardet}.

\begin{lemma} \label{ar1:Lem:SSm} Under the assumptions of 
Proposition \ref{ar1:Prop:mBICBardet} with $SS_m$ given by \eqref{ar1:Eq:SSm}, we have, for any positive $m$,
$$
SS_m(z, \overline{\rho}_n) = SS_m(z, \rho^{\star}) + O_P(1),\textrm{ as } n\to\infty\;.
$$
\end{lemma}

\begin{lemma} \label{ar1:Lem:SSmstar} Under the assumptions of Proposition
\ref{ar1:Prop:mBICBardet} with $SS_m$ given by \eqref{ar1:Eq:SSm}, we have,
for any positive $m$,
$$
SS_m(z, \rho^{\star})^{-1} = O_P(n^{-1}),\textrm{ as } n\to\infty\;.
$$
\end{lemma}

%%%%%%%%%%%%%%%%%%%%%%%%%%%%%%%%%%%%%%%%%%%%%%%%%%%%%%%%%%%%%%%%%%%%%%%%%%%%%% 
\begin{proof}[Proof of Lemma \ref{ar1:Lem:SSm}]
 The proof of this Lemma follows exactly this of Lemma \ref{ar1:Lem:SSmY}. The difference is that, in \eqref{ar1:eq:bkw}, the term $\Delta^{\star}$ appearing in the decomposition \eqref{ar1:eq:dec:second:terme} vanishes.
\end{proof}

%%%%%%%%%%%%%%%%%%%%%%%%%%%%%%%%%%%%%%%%%%%%%%%%%%%%%%%%%%%%%%%%%%%%%%%%%%%%%% 
\begin{proof}[Proof of Lemma \ref{ar1:Lem:SSmstar}]
We first define 
$$
SS_m \left(z, \rho, \boldsymbol{t}\right) = \underset{\delta}{\argmin } SS_m \left(z, \rho, \delta, \boldsymbol{t} \right).
$$ 
We have, for any positive $M$, 
\begin{eqnarray*}
 P\left(\frac{n}{SS_m(z, \rho^{\star})} > M \right) 
 & \leq & P\left( \left\{\frac{SS_m(z, \rho^{\star})}{SS_m(z, \rho^{\star}, \boldsymbol{t^{\star}})} > 1 \right\} \bigcap \left\{\frac{n}{SS_m(z, \rho^{\star})} > M\right\} \right) \\
  & & + P\left( \left\{\frac{SS_m(z, \rho^{\star})}{SS_m(z, \rho^{\star}, \boldsymbol{t^{\star}})} < 1 \right\} \bigcap \left\{\frac{n}{SS_m(z, \rho^{\star})} > M\right\} \right) \\
  & \leq & P\left(\frac{n}{SS_m(z, \rho^{\star}, \boldsymbol{t^{\star}})} > M \right) + P\left(\frac{SS_m(z, \rho^{\star})}{SS_m(z, \rho^{\star}, \boldsymbol{t^{\star}})} < 1 \right).
\end{eqnarray*}
Under the assumptions of Proposition \ref{ar1:Prop:Segment}, a by product of the proof of Theorem 3 in \textcite{LM} is that
$$
P\left(\frac{SS_m(z, \rho^{\star})}{SS_m(z, \rho^{\star}, \boldsymbol{t^{\star}})} < 1 \right) = P\left(SS_m(z, \rho^{\star}) - SS_m(z, \rho^{\star}, \boldsymbol{t^{\star}}) < 0 \right) 
\leq \kappa n^{-\alpha},
$$
where $\kappa$ is a positive constant depending on $\boldsymbol{\delta^{\star}}$ and $\boldsymbol{t^{\star}}$, and $\alpha$ is a positive constant. 
Furthermore, as $\sigma^{\star -2}SS_m(z, \rho^{\star}, \boldsymbol{t^{\star}})$ has a $\chi^2_{n-m-1}$ distribution, 
$n^{-1}SS_m(z, \rho^{\star}, \boldsymbol{t^{\star}})=\sigma^{\star 2}+o_P(1)$ and thus {$n^{-1} SS_m(z, \rho^{\star}, \boldsymbol{t^{\star}})=O_P(1)$}, which concludes the proof.
\end{proof}

\begin{proof}[Proof of Proposition \ref{ar1:Prop:mBICBardet}]
We have to prove that, for a given positive $m$, $C_m(z, \rho^{\star}) - C_m(z, \overline{\rho}_n) = O_P(1)$. 
Observe that, since $\widehat{\tau}_k(z, \rho) = \widehat{t}_k(z, \rho) /n$, 
\begin{eqnarray} \label{ar1:Eq:DecompNkZ}
& & \sum_{k=0}^m \log n_k(\widehat{t}(z, \overline{\rho}_n)) - \sum_{k=0}^m \log
n_k(\widehat{t}(z, {\rho}^{\star})) \nonumber \\
& = & \sum_{k=0}^m \log (\widehat{\tau}_{k+1}(z, \overline{\rho}_n)-\widehat{\tau}_{k}(z, \overline{\rho}_n))- 
\sum_{k=0}^m \log (\widehat{\tau}_{k+1}(z, {\rho}^{\star})-\widehat{\tau}_{k}(z, {\rho}^{\star})).
\end{eqnarray}
By Proposition  \ref{ar1:Prop:Segment}, both quantities of the previous equation converge in probability
to $$\sum_{k=0}^m \log (\tau^{\star}_{k+1}-\tau^{\star}_{k}) \,$$
thus
\begin{equation} \label{ar1:Eq:CvgceNkZ}
\sum_{k=0}^m \log n_k(\widehat{t}(z, \overline{\rho}_n))- \sum_{k=0}^m \log
n_k(\widehat{t}(z, {\rho}^{\star}))=O_P(1). 
\end{equation}
Further note that
$$
\log {SS}_m(z, \overline{\rho}_n) - \log {SS}_m(z, {\rho}^{\star})
=\log\left(\frac{{SS}_m(z, \overline{\rho}_n)}{{SS}_m(z, {\rho}^{\star})}\right) 
= R\left(\frac{{SS}_m(z, \overline{\rho}_n)-{SS}_m(z, {\rho}^{\star})}{{SS}_m(z, {\rho}^{\star})}\right),
$$
where $R(x)=\log(1+x)$.
Lemma \ref{ar1:Lem:SSm} states that ${SS}_m(z, \overline{\rho}_n)-{SS}_m(z, {\rho}^{\star}) = O_P(1)$ and Lemma \ref{ar1:Lem:SSmstar} that $[{SS}_m(z, {\rho}^{\star})]^{-1} = O_P(n^{-1})$ so, by \textcite[Lemma 2.12]{van}, we get that
$$
\log {SS}_m(z, \overline{\rho}_n) - \log {SS}_m(z, {\rho}^{\star})
= O_P(n^{-1}).
$$
Hence
$$
\frac{n-m+1}{2} \log {SS}_m(z, \overline{\rho}_n) - \frac{n-m+1}{2} \log {SS}_m(z, {\rho}^{\star}) =
O_P(1),
$$
which with (\ref{ar1:Eq:CvgceNkZ}) concludes the proof of Proposition \ref{ar1:Prop:mBICBardet}.
\end{proof}

%%%%%%%%%%%%%%%%%%%%%%%%%%%%%%%%%%%%%%%%%%%%%%%%%%%%%%%%%%%%%%%%%%%%%%%%%%%%%%%%%%%%%%%%%%%%%
\subsection{Proof of Proposition \ref{ar1:Prop:mBIC}}\label{ar1:proof:Prop:mBIC}
We first give some lemmas which are useful for the proof of Proposition \ref{ar1:Prop:mBIC}.

\begin{lemma} \label{ar1:Lem:SSmY} Under the assumptions of 
Proposition \ref{ar1:Prop:mBICBardet} with $SS_m$ given by \eqref{ar1:Eq:SSm}, we have, for any positive $m$,
$$
SS_m(y, \overline{\rho}_n) = SS_m(y, \rho^{\star}) + O_P(1),\textrm{ as } n\to\infty\;.
$$
\end{lemma}

\begin{lemma} \label{ar1:Lem:SmYZ}
  If $(y_0, \dots y_n)$ is defined by \eqref{ar1:eq:modele_new} and $(z_0, \dots z_n)$ is defined as in Lemma \ref{ar1:Lem:YZ}, then 
  $$
  SS_m(y, {\rho}^{\star}) = SS_m(z, {\rho}^{\star}) + O_P(1),\textrm{ as } n\to\infty\;.
  $$
\end{lemma}

\begin{lemma} \label{ar1:Lem:OP1}
  Let  $(X_n)$ and $(Y_n)$ be two sequences of rv's such that $X_n - Y_n = O_P(1)$. If $Y_n ^{-1} = O_P(n^{-1})$ then $X_n ^{-1} = O_P(n^{-1})$.
\end{lemma}

%%%%%%%%%%%%%%%%%%%%%%%%%%%%%%%%%%%%%%%%%%%%%%%%%%%%%%%%%%%%%%%%%%%%%%%%%%%%%% 
\begin{proof}[Proof of Lemma \ref{ar1:Lem:SSmY}]
Using the matrix notations from the proof of Lemma \ref{ar1:Lem:Delta_order}, we have
$$
SS_m(y, \rho^{\star}) = \min_{T, \delta} \Vert y - \rho^{\star} By - T \delta \Vert^2, 
\qquad
SS_m(y, \overline{\rho}_n) = \min_{T, \delta} \Vert y - \overline{\rho}_n  By - T \delta \Vert^2,
$$
where all minimizations are achieved over all segmentations with $m$ change points belonging to $\mathcal{A}_{n,m}$. 
Let us define $(\widehat{T}^{\star}, \widehat{\delta}^{\star})$
and $(\overline{T}, \overline{\delta})$ by 
\begin{equation*}
(\widehat{T}^{\star}, \widehat{\delta}^{\star}) = \argmin_{T, \delta} \Vert y - \rho^{\star}By - T\delta \Vert, 
\qquad
(\overline{T}, \overline{\delta}) = \argmin_{T, \delta} \Vert y - \overline{\rho}_n By - T\delta \Vert.
\end{equation*}
Note that $\widehat{T}^{\star}$ and $\overline{T}$ refer to $\widehat{t}(y, \rho^{\star})$ and $\widehat{t}(y, \overline{\rho}_n)$, respectively. We have 
\begin{eqnarray} \label{ar1:Eq:UpperBoundSSdiff}
 \left| SS_m(y, \overline{\rho}_n) - SS_m(y, \rho^{\star}) \right| 
 & = &  \left| \min_{T, \delta} \Vert y - \overline{\rho}_n By - T\delta \Vert^2 - \min_{T, \delta} \Vert y - \rho^{\star} By - T\delta \Vert^2 \right| \nonumber \\
 & \leq & 
 \max \left( \left| \Vert y - \overline{\rho}_n By - \widehat{T}^{\star}\widehat{\delta}^{\star} \Vert^2 - \Vert y - \rho^{\star}By - \widehat{T}^{\star}\widehat{\delta}^{\star} \Vert^2 \right|, \right. \nonumber\\
  & & \qquad \left. \left| \Vert y - \overline{\rho}_n By - \overline{T}\,\overline{\delta} \Vert^2 - \Vert y - \rho^{\star}By - \overline{T}\,\overline{\delta} \Vert^2 \right| \right).
\end{eqnarray}
We now have to prove that this upper bound is $O_P(1)$. We first prove it for the second term of in the right-hand side of \eqref{ar1:Eq:UpperBoundSSdiff}. To do so, observe that
$\Vert y - \overline{\rho}_n By - \overline{T}\,\overline{\delta} \Vert^2
=\Vert y - \rho^{\star}By - \overline{T}\,\overline{\delta}+(\rho^{\star}-\overline{\rho}_n) By\Vert^2$. Thus,
$$
\Vert y - \overline{\rho}_n By - \overline{T}\overline{\delta} \Vert^2 - \Vert y - \rho^{\star}By - \overline{T}\overline{\delta} \Vert^2 
=(\overline{\rho}_n  - \rho^{\star})^2 \Vert By\Vert^2 +2(\rho^{\star}-\overline{\rho}_n)\langle By,y - \rho^{\star}By - \overline{T}\,\overline{\delta} \rangle.
$$
Since, by (\ref{ar1:eq:modele_matriciel}) and Lemma \ref{ar1:Lem:YZ}, $y - \rho^{\star}By - \overline{T}\,\overline{\delta}
=\epsilon - \Delta^{\star} + (T^{\star}\delta^{\star}-\overline{T}\,\overline{\delta})=\epsilon- \Delta^{\star}
+T^{\star}(\delta^{\star}-\overline{\delta})+(T^{\star}-\overline{T})\overline{\delta}$, where $\Delta^{\star}$ is the $n$-dimensional vector with entries $\Delta^{\star}_i$, we get
\begin{multline}\label{ar1:eq:dec:second:terme}
\Vert y - \overline{\rho}_n By - \overline{T}\,\overline{\delta} \Vert^2 - \Vert y - \rho^{\star}By - \overline{T}\,\overline{\delta} \Vert^2\\
=(\overline{\rho}_n  - \rho^{\star})^2 \Vert By\Vert^2 
+ 2 (\rho^{\star}- \overline{\rho}_n ) \left(\langle By,\epsilon  \rangle + \langle By,T^{\star} (\delta^{\star} - \overline{\delta} )  \rangle 
+ \langle By,(T^{\star}-\overline{T}) \overline{\delta}  \rangle - \langle By, \Delta^{\star}\rangle \right).
\end{multline}
Let us now prove that each term in the right-hand side of (\ref{ar1:eq:dec:second:terme}) is $O_P(1)$.
\begin{enumerate}[($a$)]
\item Let us study the first term of (\ref{ar1:eq:dec:second:terme}).
Using Lemma \ref{ar1:lem:rateXY} and (\ref{ar1:eq:hypRhoRate}) we get that 
  \begin{equation}\label{ar1:Eq:rhoXnorm}
  (\overline{\rho}_n -\rho^{\star})^2 \Vert By\Vert^2 = O_P(1).
  \end{equation}
\item Let us now study the second term of (\ref{ar1:eq:dec:second:terme}). Observe that 
$
\left\langle By,\epsilon\right\rangle = \sum_{i=1}^n y_{i-1}\epsilon_i=\sum_{i=1}^n (y_{i-1}-\PE(y_{i-1}))\epsilon_i+\sum_{i=1}^n \PE(y_{i-1})\epsilon_i.
$
By using the Central limit theorem for  iid rv's and since there is a finite number of change-points, the second term
is $O_P(\sqrt{n})$. As for the first term, since $(y_{i-1}-\PE(y_{i-1}))$ is a causal AR(1) process, then by using the beginning of the proof of Proposition 8.10.1 of \textcite{brockwell}, we get
that $\sum_{i=1}^n (y_{i-1}-\PE(y_{i-1}))\epsilon_i=O_P (\sqrt{n})$. Thus,
  \begin{equation} \label{ar1:Eq:CrossProd1}  
  \left\langle By,\epsilon\right\rangle %= \sum_{i=1}^n y_{i-1}\epsilon_i 
= O_P (\sqrt{n}).
 \end{equation}
  Furthermore, we have $\Vert T^{\star} ( \delta^{\star} - \overline{\delta} ) \Vert^2 = \sum_{k=0}^{m}\left(t_{k+1}^{\star}-t_k^{\star}\right) (\delta^{\star}_k -\overline{\delta}_k)^2$ 
 where each term of the sum is $O_P(1)$, thanks to Proposition \ref{ar1:Prop:Segment2}, and so is the sum. 
Now using Lemma \ref{ar1:lem:rateXY} and the Cauchy-Schwarz inequality, we get 
\begin{equation} \label{ar1:Eq:CrossProd2}  
  \langle By, T^{\star} ( \delta^{\star} - \overline{\delta} )  \rangle = O_P(\sqrt{n}).
  \end{equation}
  The convergence rate of $\widehat{t}(y,\overline{\rho}_n)$ given in Proposition \ref{ar1:Prop:Segment2} ensures that, for any $\varepsilon>0$ there exists a positive $M$ 
such that each column of $(T^{\star} - \overline{T})$ has at most $M$ non-zero coefficients with probability greater than $1-\varepsilon$. 
By using Proposition \ref{ar1:Prop:Segment2}, we obtain that with probability greater than $1-\varepsilon$
  \begin{equation}\label{ar1:eq:T*-Tbar}
  \Vert(T^{\star} - \overline{T}) \overline{\delta} \Vert^2 \leq M \sum_k \overline{\delta}_k^2 =2 M \sum_k (\overline{\delta}_k-\delta^{\star}_k)^2
+2M \sum_k {\delta^{\star}_k}^2\leq MM',
\end{equation}
where $M'$ is a positive constant. 
By the Cauchy-Schwarz inequality, (\ref{ar1:eq:T*-Tbar}) and Lemma \ref{ar1:lem:rateXY}, we get 
  \begin{equation} \label{ar1:Eq:CrossProd3}  
  \langle By, (T^{\star} - \overline{T}) \overline{\delta}  \rangle = O_P (\sqrt{n}).
  \end{equation}
  As $\Delta^{\star}$ has only $m$ non-zero entries, $\langle By, \Delta^{\star}\rangle$ is the sum of $m$ Gaussian rv's and is therefore $O_P(1)$.
  
  Thus, combining \eqref{ar1:Eq:CrossProd1}, \eqref{ar1:Eq:CrossProd2} and \eqref{ar1:Eq:CrossProd3} with (\ref{ar1:eq:hypRhoRate}), we get
  $$
  (\rho^{\star}- \overline{\rho}_n ) \left(\langle By,\epsilon  \rangle + \langle By,T^{\star} (\delta^{\star} - \overline{\delta} )  \rangle + \langle By,(T^{\star} - \overline{T}) \overline{\delta}  \rangle -  \langle By, \Delta^{\star}\rangle \right) = O_P(1).
  $$
\end{enumerate}

To complete the proof, we need to consider the first term of \eqref{ar1:Eq:UpperBoundSSdiff}.
As $\rho^{\star}$ satisfies the same assumptions as $\overline{\rho}_n$, using the same line of reasoning as for the second term holds so we get
$$
\Vert y - \overline{\rho}_n By - \widehat{T}^{\star}\widehat{\delta}^{\star} \Vert^2 - \Vert y - \rho^{\star}By - \widehat{T}^{\star}\widehat{\delta}^{\star} \Vert^2 = O_P(1).
$$

\end{proof}

%%%%%%%%%%%%%%%%%%%%%%%%%%%%%%%%%%%%%%%%%%%%%%%%%%%%%%%%%%%%%%%%%%%%%%%%%%%%%% 
\begin{proof}[Proof of Lemma \ref{ar1:Lem:SmYZ}] 
The proof follows the same line of reasoning as the proof of Lemma \ref{ar1:Lem:SSmY}.

Let us define $(\widehat{T}^y, \widehat{\delta}^y)$
and $(\widehat{T}^z, \widehat{\delta}^z)$ by 
\begin{equation*}
(\widehat{T}^y, \widehat{\delta}^y)
= \argmin_{T, \delta} 
\Vert y - \rho^{\star} By - T \delta \Vert^2,
\qquad
(\widehat{T}^z, \widehat{\delta}^z)
= \argmin_{T, \delta} 
\Vert z - \rho^{\star} Bz - T \delta \Vert^2.
\end{equation*}
We have 
\begin{multline*} 
\left|SS_m(y, \rho^{\star}) - SS_m(z, \rho^{\star}) \right\| 
 \leq 
 \max \left( \left| \Vert y - \rho^{\star} By - \widehat{T}^y \widehat{\delta}^y \Vert^2 - \Vert z - \rho^{\star}Bz - \widehat{T}^y \widehat{\delta}^y \Vert^2 \right|, \right. \\
 \left. \left| \Vert y - \rho^{\star} By - \widehat{T}^z \widehat{\delta}^z \Vert^2 - \Vert z - \rho^{\star}Bz - \widehat{T}^z \widehat{\delta}^z \Vert^2 \right| \right).
\end{multline*}
According to Lemma \ref{ar1:Lem:YZ}, we have $y - \rho^{\star} By = z - \rho^{\star} Bz - \Delta^{\star}$ where $\Delta^{\star}=(\Delta_i^{\star})$. As for the first term
\begin{multline*}
\Vert y - \rho^{\star} By - \widehat{T}^y \widehat{\delta}^y \Vert^2 - \Vert z - \rho^{\star}Bz - \widehat{T}^y \widehat{\delta}^y \Vert^2 \\
= \Vert \Delta^{\star} \Vert^2 
- 2 \left(\langle \Delta^{\star},\epsilon \rangle + \langle \Delta^{\star}, T^{\star} (\delta^{\star} - \widehat{\delta}^y )  \rangle 
+ \langle \Delta^{\star},(T^{\star}-\widehat{T}^y) \widehat{\delta}^y \rangle \right),
\end{multline*}
the first term of which is a constant and all other terms being $O_P(1)$, which can be proved following the same line as the proof of Lemma \ref{ar1:Lem:SSmY}. The control of $\Vert y - \rho^{\star} By - \widehat{T}^z \widehat{\delta}^z \Vert^2 - \Vert z - \rho^{\star}Bz - \widehat{T}^z \widehat{\delta}^z \Vert^2$ follows the same lines.
  \end{proof}

%%%%%%%%%%%%%%%%%%%%%%%%%%%%%%%%%%%%%%%%%%%%%%%%%%%%%%%%%%%%%%%%%%%%%%%%%%%%%% 
\begin{proof}[Proof of Lemma \ref{ar1:Lem:OP1}]
Observe that 
$$X_n^{-1}=\left(Y_n+(X_n-Y_n)\right)^{-1}=Y_n^{-1}\left(1+Y_n^{-1}(X_n-Y_n)\right)^{-1}\; .$$
Since, by assumption, $Y_n^{-1}(X_n-Y_n)=O_P(n^{-1})$, the terms inside
the parentheses converges in probability to one. Thus, $\left(1+Y_n^{-1}(X_n-Y_n)\right)^{-1}$ is in particular $O_P(1)$ which concludes the proof.
\end{proof}

\begin{proof}[Proof of Proposition \ref{ar1:Prop:mBIC}]
   As for the proof of Proposition \ref{ar1:Prop:mBICBardet}, denoting $\widehat{\tau}_k(y, \rho) = \widehat{t}_k(y, \rho) /n$, the decomposition \eqref{ar1:Eq:DecompNkZ} still holds, replacing $z$ with $y$. Then, by Proposition~\ref{ar1:Prop:Segment2}, we have
   $$
   \sum_{k=0}^m \log n_k(\widehat{t}(y, \overline{\rho}_n))- \sum_{k=0}^m \log
   n_k(\widehat{t}(y, {\rho}^{\star}))=O_P(1). 
   $$
   For a process $y$ under Model~\eqref{ar1:eq:modele_new}, we construct a process $z$ under Model~\eqref{ar1:eq:bkw} using Lemma~\ref{ar1:Lem:YZ}. The proof relies on the fact that $y$ inherits some properties of $z$. Again, we note that
   $$
   \log {SS}_m(y, \overline{\rho}_n) - \log {SS}_m(y, {\rho}^{\star})
    = R\left(\frac{{SS}_m(y, \overline{\rho}_n)-{SS}_m(y, {\rho}^{\star})}{{SS}_m(y, {\rho}^{\star})}\right).
   $$
  Lemma \ref{ar1:Lem:SSmY} states that ${SS}_m(y, \overline{\rho}_n)-{SS}_m(y, {\rho}^{\star}) = O_P(1)$. 
  To conclude the proof we need to further show that $[{SS}_m(y, {\rho}^{\star})]^{-1} = O_P(n^{-1})$. We first show that $[{SS}_m(y, {\rho}^{\star}) - {SS}_m(z, {\rho}^{\star})] = O_P(1)$ in Lemma~\ref{ar1:Lem:SmYZ} and, because $[{SS}_m(z, {\rho}^{\star})]^{-1} = O_P(n^{-1})$, we conclude using Lemma~\ref{ar1:Lem:OP1}.
\end{proof}

%%% Local Variables:
%%% mode: latex
%%% eval: (TeX-PDF-mode 1)
%%% TeX-master: "article.tex"
%%% ispell-local-dictionary: "en_US"
%%% eval: (flyspell-mode 1)
%%% End: 
