# Supplementary material for: A robust approach for estimating change-points in the mean of an AR(p) process
Source: arXiv:1509.00899 source file (2015-09-02)
Supplement: Supplementary file 3 [file AppSec2.tex]

\subsection{Proof of Proposition \ref{ar1:prop:correlation}}\label{ar1:proof:corr_tcl}


Let $F_1$ and $F_2$ denote the cumulative distribution functions (cdf) of 
$\left(\left|y_{i+1}-y_i\right|\right)$ for $i\neq t_{n,1}^{\star},\dots,t_{n,m^{\star}}^{\star}$ and $\left(|y_{i+2}-y_i|\right)$
for $i\neq t_{n,1}^{\star}-1,\dots,t_{n,m^{\star}}^{\star}-1$,
respectively. By  (\ref{ar1:eq:modele_new}), 
$(y_i-\PE(y_i))_{0\leq i\leq n}$ are $(n+1)$ observations of a AR(1) stationary Gaussian process thus for any $i\neq t_{n,1}^{\star},\dots,t_{n,m^{\star}}^{\star}$, 
$(y_{i+1}-y_i)$ and for any $i\neq t_{n,1}^{\star}-1,\dots,t_{n,m^{\star}}^{\star}-1$, $(y_{i+2}-y_i)$ are 
zero-mean Gaussian rv's with variances equal to
$2\sigma^{\star 2}/(1+\rho^{\star})$ and $2\sigma^{\star 2}$, respectively.
Hence, for all $t$ in $\rset$,
\begin{equation}\label{ar1:eq:def:F1:F2}
F_1:t\mapsto 2\Phi\left(t\sqrt{\frac{1+\rho^{\star}}{2\sigma^{\star 2}}}\right)-1
\textrm{ and } F_2:t\mapsto 2\Phi\left(t\sqrt{\frac{1}{2\sigma^{\star 2}}}\right)-1\;,
\end{equation}
where $\Phi$ denotes the cumulative distribution function of a standard Gaussian rv.

Let also denote by $F_{1,n}$ and $F_{2,n-1}$ the empirical cumulative distribution functions of
$\left(|y_{i+1}-y_i|\right)_{0\leq i\leq n-1}$ and $\left(|y_{i+2}-y_i|\right)_{0\leq i\leq n-2}$,
respectively. Observe that for all $t$ in $\mathbb{R}$,
\begin{multline}\label{ar1:eq:cdf1}
\sqrt{n}(F_{1,n}(t)-F_1(t))=\frac{1}{\sqrt{n}}\sum_{i=0}^{n-1} \left(\1_{\{|y_{i+1}-y_i|\leq t\}}-F_1(t)\right)\\
=\frac{1}{\sqrt{n}}\sum_{i\in \{t_{n,1}^{\star},\dots,t_{n,m^{\star}}^{\star}\}}\left(\1_{\{|y_{i+1}-y_i|\leq t\}}-F_1(t)\right)
+\frac{1}{\sqrt{n}}\sum_{\stackrel{0\leq i\leq n-1}{i \notin \{t_{n,1}^{\star},\dots,t_{n,m^{\star}}^{\star}\}}} \left(\1_{\{|y_{i+1}-y_i|\leq t\}}-F_1(t)\right)\\
=\frac{1}{\sqrt{n}}\sum_{0\leq i\leq n-1} \left(\1_{\{|z_i|\leq t\}}-F_1(t)\right)+R_n(t)\;,
\end{multline}
where $\sup_{t\in\rset} |R_n(t)|=o_p(1)$, the $z_i=y_{i+1}-y_i$ except for $i =t_{n,1}^{\star},\dots,t_{n,m^{\star}}^{\star}$, where
$z_i=\eta_{i+1}-\eta_i$, $(\eta_i)$ being defined in (\ref{ar1:eq:ar1}).

Thus, by using the theorem of \textcite{CM}\footnote{See Theorem~\ref{th:CM} of this document.}, we obtain that the first term in the right-hand side of (\ref{ar1:eq:cdf1}) 
converges in distribution to a zero-mean Gaussian process $G$ in the
space of c\`adl\`ag functions equipped with the uniform norm. Since the second term in the right-hand side 
tends uniformly to zero in probability, we get that $\sqrt{n}(F_{1,n}-F_1)$ converges in distribution to a zero-mean Gaussian process in the
space of c\`adl\`ag functions equipped with the uniform norm
and that the same holds for $\sqrt{n-1}(F_{2,n-1}-F_2)$.

By Lemma 21.3 of \textcite{van} the quantile function $T: F\mapsto F^{-1}(1/2)$
is Hadamard differentiable at $F$ tangentially to the set of c\`adl\`ag functions $h$ that are continuous at
$F^{-1}(1/2)$ with derivative $T'_F(h)=-h(F^{-1}(1/2))/F'(F^{-1}(1/2))$.
By applying the functional delta method \parencite[Theorem 20.8]{van}\footnote{See Theorem~\ref{th:delta_methode_fonctionnelle} of this document.}, we get that
$\sqrt{n}(T(F_{1,n})-T(F_1))$ converges in distribution to $T'_{F_1}(G)$. Moreover, by the 
Continuous mapping theorem, it is the same for $T'_{F_1}\left\{\sqrt{n}(F_{1,n}-F_1)\right\}$. Thus,
\begin{multline*}%\label{ar1:eq:expansion_F1}
\sqrt{n}\left(F^{-1}_{1,n}(1/2)-F_1^{-1}(1/2)\right)
=T'_{F_1}\left\{\sqrt{n}(F_{1,n}-F_1)\right\}+o_p(1)\\
=-\frac{1}{\sqrt{n}}\frac{\sum_{i=0}^{n-1}\left(\1_{\{|y_{i+1}-y_i|\leq F_1^{-1}(1/2)\}}-1/2\right)}
{F_1'(F_1^{-1}(1/2))}+o_p(1)\;.
\end{multline*}
In the same way,
\begin{multline*}%\label{ar1:eq:expansion_F2}
\sqrt{n-1}\left(F^{-1}_{2,n-1}(1/2)-F_2^{-1}(1/2)\right)=\\
-\frac{1}{\sqrt{n-1}}\frac{\sum_{i=0}^{n-2}\left(\1_{\{|y_{i+2}-y_i|\leq F_2^{-1}(1/2)\}}-1/2\right)}
{F_2'(F_2^{-1}(1/2))}+o_p(1)\;,
\end{multline*}

By applying the Delta method \parencite[Theorem 3.1]{van}\footnote{See Theorem~\ref{th:DeltaMethode} of this document.} with the transformation $f(x)=x^2$, we get
\begin{multline*}%\label{ar1:eq:expansion_F1_square}
\sqrt{n}\left(F^{-1}_{1,n}(1/2)^2-F_1^{-1}(1/2)^2\right)=\\
-\frac{2 F_1^{-1}(1/2)}{\sqrt{n}}\frac{\sum_{i=0}^{n-1}\left(\1_{\{|y_{i+1}-y_i|\leq F_1^{-1}(1/2)\}}-1/2\right)}
{F_1'(F_1^{-1}(1/2))}+o_p(1)\;,
\end{multline*}
\begin{multline*}%\label{ar1:eq:expansion_F2_square}
\sqrt{n-1}\left(F^{-1}_{2,n-1}(1/2)^2-F_2^{-1}(1/2)^2\right)=\\
-\frac{2 F_2^{-1}(1/2)}{\sqrt{n-1}}\frac{\sum_{i=0}^{n-2}\left(\1_{\{|y_{i+2}-y_i|\leq F_2^{-1}(1/2)\}}-1/2\right)}
{F_2'(F_2^{-1}(1/2))}+o_p(1)\;,
\end{multline*}
Note that by (\ref{ar1:eq:def:F1:F2}), we obtain that
\begin{equation}\label{ar1:eq:F1-1:F2-1}
F_1^{-1}(1/2)=\sqrt{\frac{2\sigma^{\star 2}}{1+\rho^{\star}}}\Phi^{-1}(3/4) \textrm{ and } F_2^{-1}(1/2)=\sqrt{2\sigma^{\star 2}}\Phi^{-1}(3/4)\;.
\end{equation}
Moreover,
\begin{equation}\label{ar1:eq:F1prime:F2prime}
F_1'(F_1^{-1}(1/2))=2\sqrt{\frac{1+\rho^{\star}}{2\sigma^{\star 2}}}\varphi\left(\Phi^{-1}(3/4)\right)   
\textrm{ and } F_2'(F_2^{-1}(1/2))=2\sqrt{\frac{1}{2\sigma^{\star 2}}}\varphi\left(\Phi^{-1}(3/4)\right)\;,
\end{equation}
where $\varphi$ denotes the probability distribution function of a standard Gaussian rv.

Observe that $\sqrt{n}(\widetilde{\rho}_n - \rho^{\star})$ can be rewritten as follows:
\begin{multline}\label{ar1:eq:expansion_rhotilde_1}
\sqrt{n}(\widetilde{\rho}_n - \rho^{\star})=\sqrt{n}\;\frac{F^{-1}_{2,n}(1/2)^2-(1+\rho^{\star}) F^{-1}_{1,n}(1/2)^2}{F^{-1}_{1,n}(1/2)^2}\\
=\sqrt{n}\;\frac{\left(F^{-1}_{2,n-1}(1/2)^2-F_2^{-1}(1/2)^2\right) -(1+\rho^{\star}) \left(F^{-1}_{1,n}(1/2)^2-F_1^{-1}(1/2)^2\right)}{F^{-1}_{1,n}(1/2)^2}\\
+\sqrt{n}\;\frac{F_2^{-1}(1/2)^2-(1+\rho^{\star})F_1^{-1}(1/2)^2}{F^{-1}_{1,n}(1/2)^2}\;.
\end{multline}
By (\ref{ar1:eq:F1-1:F2-1}) the last term in the right-hand side of (\ref{ar1:eq:expansion_rhotilde_1}) is equal to zero. Thus,
\begin{multline*}
F^{-1}_{1,n}(1/2)^2 \sqrt{n}(\widetilde{\rho}_n - \rho^{\star})=\\
\frac{1}{\sqrt{n-1}}\sum_{i=0}^{n-2} \left\{a_2\left(\1_{\{|y_{i+2}-y_i|\leq F_2^{-1}(1/2)\}}-1/2\right)
-a_1 (1+\rho^{\star})\left(\1_{\{|y_{i+1}-y_i|\leq F_1^{-1}(1/2)\}}-1/2\right)\right\}+o_p(1)\;,
\end{multline*}
where, by (\ref{ar1:eq:F1prime:F2prime}), 
\begin{eqnarray*}
a_2 & = &-\frac{2 F_2^{-1}(1/2)}{F_2'(F_2^{-1}(1/2))}=-2\sigma^{\star 2}\frac{\Phi^{-1}(3/4)}{\varphi\left(\Phi^{-1}(3/4)\right)}\\
\textrm{ and } a_1 & = & -\frac{2F_1^{-1}(1/2)}{F_1'(F_1^{-1}(1/2))}=-\frac{2\sigma^{\star 2}}{1+\rho^{\star}}\frac{\Phi^{-1}(3/4)}{\varphi\left(\Phi^{-1}(3/4)\right)}  \;.
\end{eqnarray*}
By (\ref{ar1:eq:F1-1:F2-1}), $\sqrt{n}(\widetilde{\rho}_n - \rho^{\star})$ can thus be rewritten as follows:
\begin{equation*}
F^{-1}_{1,n}(1/2)^2 \sqrt{n}(\widetilde{\rho}_n - \rho^{\star})=\frac{2\sigma^{\star 2}\Phi^{-1}(3/4)^2}{1+\rho^\star} \frac{1}{\sqrt{n-1}}\sum_{0\leq i\leq n-2}
\Psi(\eta_i,\eta_{i+1},\eta_{i+2})+o_p(1)\;.
\end{equation*}
where $\Psi$ is defined in (\ref{ar1:eq:def_Psi}) and 
%$w_i=y_i$ except when $i=t_{n,1}^{\star},\dots,t_{n,m^{\star}}^{\star},t_{n,1}^{\star}-1,\dots,t_{n,m^{\star}}^{\star}-1$
%where $w_i=\eta_i$, where 
$(\eta_i)$ is defined in (\ref{ar1:eq:ar1}).
Since $\Psi$ is a function on $\rset^3$ with Hermite rank greater than 1 and $(\eta_i)_{i\geq 0}$ is a stationary AR(1) Gaussian process, and since $F^{-1}_{1,n}(1/2)^2$ converges in probability to $F^{-1}_{1}(1/2)^2$, (\ref{ar1:eq:tcl_rho_tilde}) follows by applying \textcite[Theorem 4]{arcones1994limit}\footnote{See Theorem~\ref{th:arcones} of this document.}, Slutsky's lemma and Equation~\eqref{ar1:eq:F1-1:F2-1}.

\subsection{Hints for \eqref{ar1:eq:rho_cauchy}}\label{ar1:subsec:hints}
Note that if $X$ has a Cauchy($x_0$,$\gamma$) distribution then the characteristic function $\varphi_X$
of $X$ can be written as
$
\varphi_X(t)=\rme^{\rmi x_0 t-\gamma |t|}.
$
Moreover, the cdf $F_X$ of $X$ is such that $F_X^{-1}(3/4)=x_0+\gamma$.
Thus, $\eta_i=\sum_{k\geq 0} (\rho^{\star})^k \varepsilon_{i-k}$ has a 
Cauchy$\left(\frac{x_0}{1-\rho^{\star}},\frac{\gamma}{1-|\rho^{\star}|}\right)$ distribution and
$(\rho^{\star} -1)\eta_i$ has a Cauchy$\left(-x_0,\frac{\gamma|\rho^{\star} -1|}{1-|\rho^{\star}|}\right)$ distribution.
Since $\eta_{i+1}-\eta_i=(\rho^{\star} -1)\eta_i+\varepsilon_i$ is a sum of two independent Cauchy rv's,
it is distributed as a Cauchy$\left(0,\gamma\left(1+\left|\frac{\rho^{\star}-1}{1-|\rho^{\star}|}\right|\right)\right)$ distribution.
In the same way, 
$\eta_{i+2}-\eta_i=({\rho^{\star}}^2 -1)\eta_i+\rho^{\star}\varepsilon_i+\varepsilon_{i+2}$ is a sum 
of three independent Cauchy rv's and has thus a Cauchy$\left(0,2\gamma(1+|\rho^{\star}|)\right)$.
Let $F_1$ and $F_2$ denote the cdf of $(\eta_{i+1}-\eta_i)$ and $(\eta_{i+2}-\eta_i)$, respectively.
By using the properties of the cdf of a Cauchy distribution, we get, on the one hand, that
$F_2^{-1}(3/4)=2\gamma(1+|\rho^{\star}|)$ and, on the other hand, that
$$
F_1^{-1}(3/4)=
\left\{
\begin{array}{cc}
2\gamma,&\textrm{if } \rho^{\star}>0\;,\\
\frac{2\gamma}{1+\rho^{\star}},&\textrm{if } \rho^{\star}<0\;.
\end{array}
\right.
$$
From this we get that
\begin{equation*}%\label{ar1:eq:lim_F2_F1}
\left(\frac{F_2^{-1}(3/4)}{F_1^{-1}(3/4)}\right)^2-1=
\left\{
\begin{array}{cc}
\rho^{\star}(2+\rho^{\star}),&\textrm{if } \rho^{\star}>0\;,\\
{\rho^{\star}}^2({\rho^{\star}}^2-2),&\textrm{if } \rho^{\star}<0\;.
\end{array}
\right.
\end{equation*}
The definition of $\widetilde{\widetilde{\rho}}_n$ comes by inverting
these last two functions.

%%% Local Variables:
%%% mode: latex
%%% eval: (TeX-PDF-mode 1)
%%% TeX-master: "article.tex"
%%% ispell-local-dictionary: "en_US"
%%% eval: (flyspell-mode 1)
%%% End:
